# Supplementary material for: A Sequential Monte Carlo Method for Data Assimilation in Subsurface Flow Systems with Hierarchical Uncertainty
Source: arXiv:2611.11681 source file (2026-11-08)
Supplement: Supplementary file 1 [file SM.tex]

\documentclass[preprint,12pt]{elsarticle}
\usepackage[T1]{fontenc}
\usepackage{geometry}
\geometry{letterpaper,margin=2.5cm}
\usepackage{graphicx}
\usepackage{booktabs,tabularx}
\usepackage[font=small,skip=5pt]{caption}
\usepackage{placeins}
\usepackage[hidelinks]{hyperref}

\renewcommand{\thesection}{S\arabic{section}}
\renewcommand{\thefigure}{S\arabic{figure}}
\renewcommand{\thetable}{S\arabic{table}}


\setcounter{topnumber}{3}
\setcounter{bottomnumber}{2}
\setcounter{totalnumber}{4}
\renewcommand{\topfraction}{.95}
\renewcommand{\bottomfraction}{.80}
\renewcommand{\textfraction}{.05}
\renewcommand{\floatpagefraction}{.60}
\setlength{\textfloatsep}{10pt plus 2pt minus 2pt}
\setlength{\floatsep}{8pt plus 2pt minus 2pt}
\setlength{\intextsep}{10pt plus 2pt minus 2pt}

\makeatletter
\setlength{\@fptop}{0pt}
\setlength{\@fpsep}{8pt plus 2pt minus 2pt}
\setlength{\@fpbot}{0pt plus 1fil}
\newenvironment{centeredfigurepage}
  {\clearpage\begingroup
   \setlength{\@fptop}{0pt plus 1fil}%
   \begin{figure}[p]\centering}
  {\end{figure}\clearpage\endgroup}
\makeatother


\begin{document}

\begin{center}

{\Large\bfseries
Supplementary Material\par}

\vspace{1.0em}

{\large\bfseries
A Sequential Monte Carlo Method for Data Assimilation in Subsurface Flow Systems with Hierarchical Uncertainty\par}

\vspace{1.2em}

{\normalsize
Wenchao Teng$^{a}$, Guido Di Federico$^{a}$, Louis J.~Durlofsky$^{a}$\par}

\vspace{0.7em}

{\small\itshape
$^{a}$Department of Energy Science and Engineering, Stanford University, Stanford, CA 94305, USA\par}

\vspace{1.0em}

\end{center}

\hrule

\vspace{1.0em}

\section*{SM overview}

Details on the flow surrogate models and data assimilation results for additional cases are provided in this SM. The SM is organized as follows. In Section~S1, we present surrogate results for pressure in the faulted carbon storage system and the network architecture for the flow surrogate developed for the channelized oil-water system. Additional results for the faulted carbon storage system, including successive data assimilation results for the case considered in the main text and results for a second synthetic true model (Case~3), are provided in Section~S2. Field-level rate predictions, which supplement the Case~2 results in Section~6 of the main text, along with results for a second synthetic channelized true model (Case~4), appear in Section~S3.


\section{Flow surrogate models}
\label{sec:sm_surrogates}

Figure~\ref{fig:pressure_comparison} presents a comparison of pressure fields from flow simulations (top row) and surrogate model predictions (bottom row) for the uppermost layer of the target aquifer at 50~years. Results for three test-set realizations are shown. The realizations exhibit different pressure distributions, with more pronounced contrasts across fault~1 (leftmost fault) in realizations~5 and~6. The flow surrogate closely reproduces the overall pressure patterns and the localized effects associated with the faults.


\begin{figure}[!htbp]
\centering
\includegraphics[width=0.71\linewidth]
{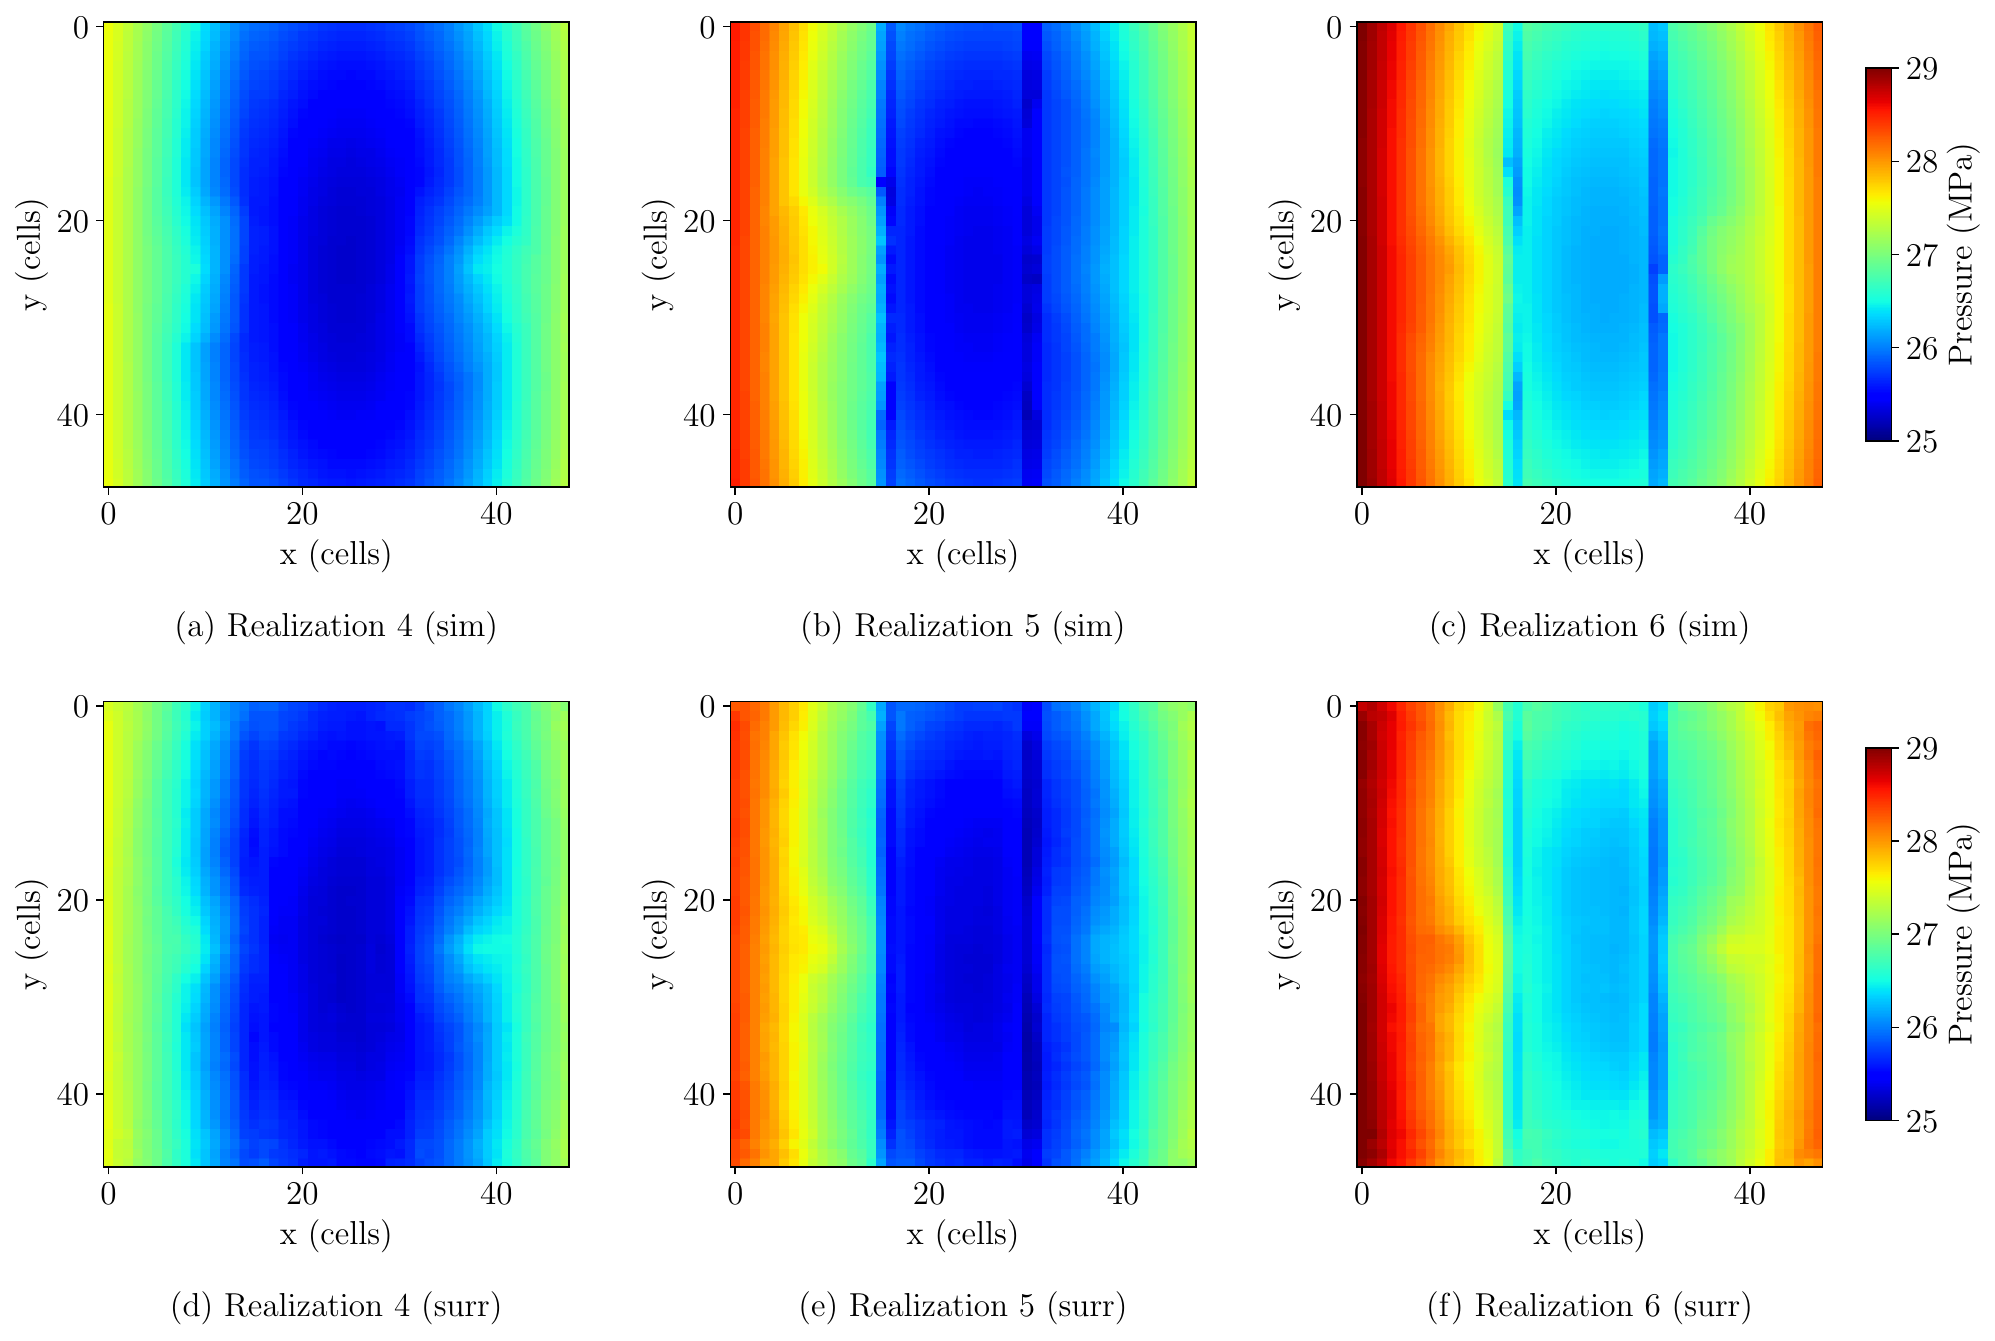}
\caption{Pressure distribution in the uppermost layer of the target aquifer at 50~years for three test-set realizations (realizations~4--6). GEOS simulation results are shown in the top row and surrogate model predictions in the bottom row.}
\label{fig:pressure_comparison}
\end{figure}


Table~\ref{tab:ow-surrogate-architecture} provides the detailed network architecture of the flow surrogate for the channelized oil-water system. This surrogate model is discussed in Section~2.2 %\ref{sec:oil_geomodel} 
of the main text. The architecture includes spatial and metaparameter encoders, attention-based feature extraction, and a recurrent temporal decoder for predicting well rates.


\begin{table}[!htbp]
\centering
\caption{Network architecture for the flow surrogate for 3D channelized oil-water systems.}
\label{tab:ow-surrogate-architecture}
\begingroup
\small
\setlength{\tabcolsep}{4.5pt}
\renewcommand{\arraystretch}{1.0}
\begin{tabularx}{\linewidth}{@{}
    >{\raggedright\arraybackslash}p{0.26\linewidth}
    >{\raggedright\arraybackslash}X
    >{\raggedleft\arraybackslash}p{0.22\linewidth}@{}}
\toprule
Network & Layer & Output size \\
\midrule
Spatial encoder
 & Input & $(128,128,32,9)$ \\
 & Residual block, 32 filters & $(128,128,32,32)$ \\
 & 2 residual blocks, 32 filters, $s=(2,2,1)$ & $(64,64,32,32)$ \\
 & 2 residual blocks, 64 filters, $s=(2,2,2)$ & $(32,32,16,64)$ \\
 & 2 residual blocks, 128 filters, $s=(2,2,2)$ & $(16,16,8,128)$ \\
 & 2 residual blocks, 256 filters, $s=(2,2,1)$ & $(8,8,8,256)$ \\
 & Multi-head self-attention, width 192 & $(8,8,8,256)$ \\
\midrule
Metaparameter encoder
 & 3 MLPs, $3\to32\to32$; MLP, $96\to128\to128$ & $(128)$ \\
\midrule
Feature extraction
 & Embedding; linear projection & $(9,128)$ \\
 & Sampling and pooling; linear $1024\to128$ & $(9,128)$ \\
 & Multi-head cross-attention, 512 tokens & $(9,128)$ \\
 & Concatenation; MLP, $512\to256\to128$ & $(9,128)$ \\
\midrule
Attention
 & Multi-head cross-attention, 3 scales & $(18,128)$ \\
 & Multi-head cross-attention & $(9,128)$ \\
 & Transformer block, 2 layers & $(9,128)$ \\
\midrule
Temporal decoder
 & Fourier features; MLP, $5\to64\to64$
 & $(30,64)$ \\
 & Concatenation; GRU, 2 layers, 128 units & $(9,30,128)$ \\
\midrule
Output
 & MLP, $128\to64\to2$ & $(6,30,2)$ \\
 & MLP, $128\to64\to1$ & $(3,30,1)$ \\
 & Softplus; concatenation & $(30,15)$ \\
\bottomrule
\end{tabularx}
\par\vspace{3pt}
\begin{minipage}{\linewidth}
\raggedright\footnotesize
Residual blocks contain two $3\times3\times3$ convolutions, group normalization, and SiLU; $s$ denotes stride. All attention modules use four heads. MLP: multilayer perceptron; GRU: gated recurrent unit.
\end{minipage}
\endgroup
\end{table}


\FloatBarrier


\section{Additional results for the faulted carbon storage system}
\label{sec:si-true-model-2}

Additional results for Case~1B, which considers observations through year~12, are presented in Fig.~\ref{fig:6t-s9-marg}. In this figure we compare the marginal posterior metaparameter distributions obtained using single-stage SMC, successive SMC, and MCMC. The MCMC calculation reached the 50-hour time limit without satisfying the convergence criterion, as noted in Section~5.2 of the main paper. In the marginal density plots in Fig.~\ref{fig:6t-s9-marg} (and in subsequent figures of this type in SM), we use $h=2h_{\mathrm{Scott}}$, as discussed in Section~5.1 in the main text. Note that $h=h_{\mathrm{Scott}}$ was used in Fig.~8. From Fig.~\ref{fig:6t-s9-marg}, we see that the three approaches provide generally consistent posterior results, with substantial reduction in predictive uncertainty relative to the prior. Some discrepancies are apparent in a few of the metaparameters ($\mu_{\log k}$, $\log_{10}(a_r)$, $k_u$, $e$), though this does not lead to significant differences in the flow responses shown in Fig.~15 in the main text.


\begin{figure}[!htbp]
\centering
\includegraphics[width=\linewidth]{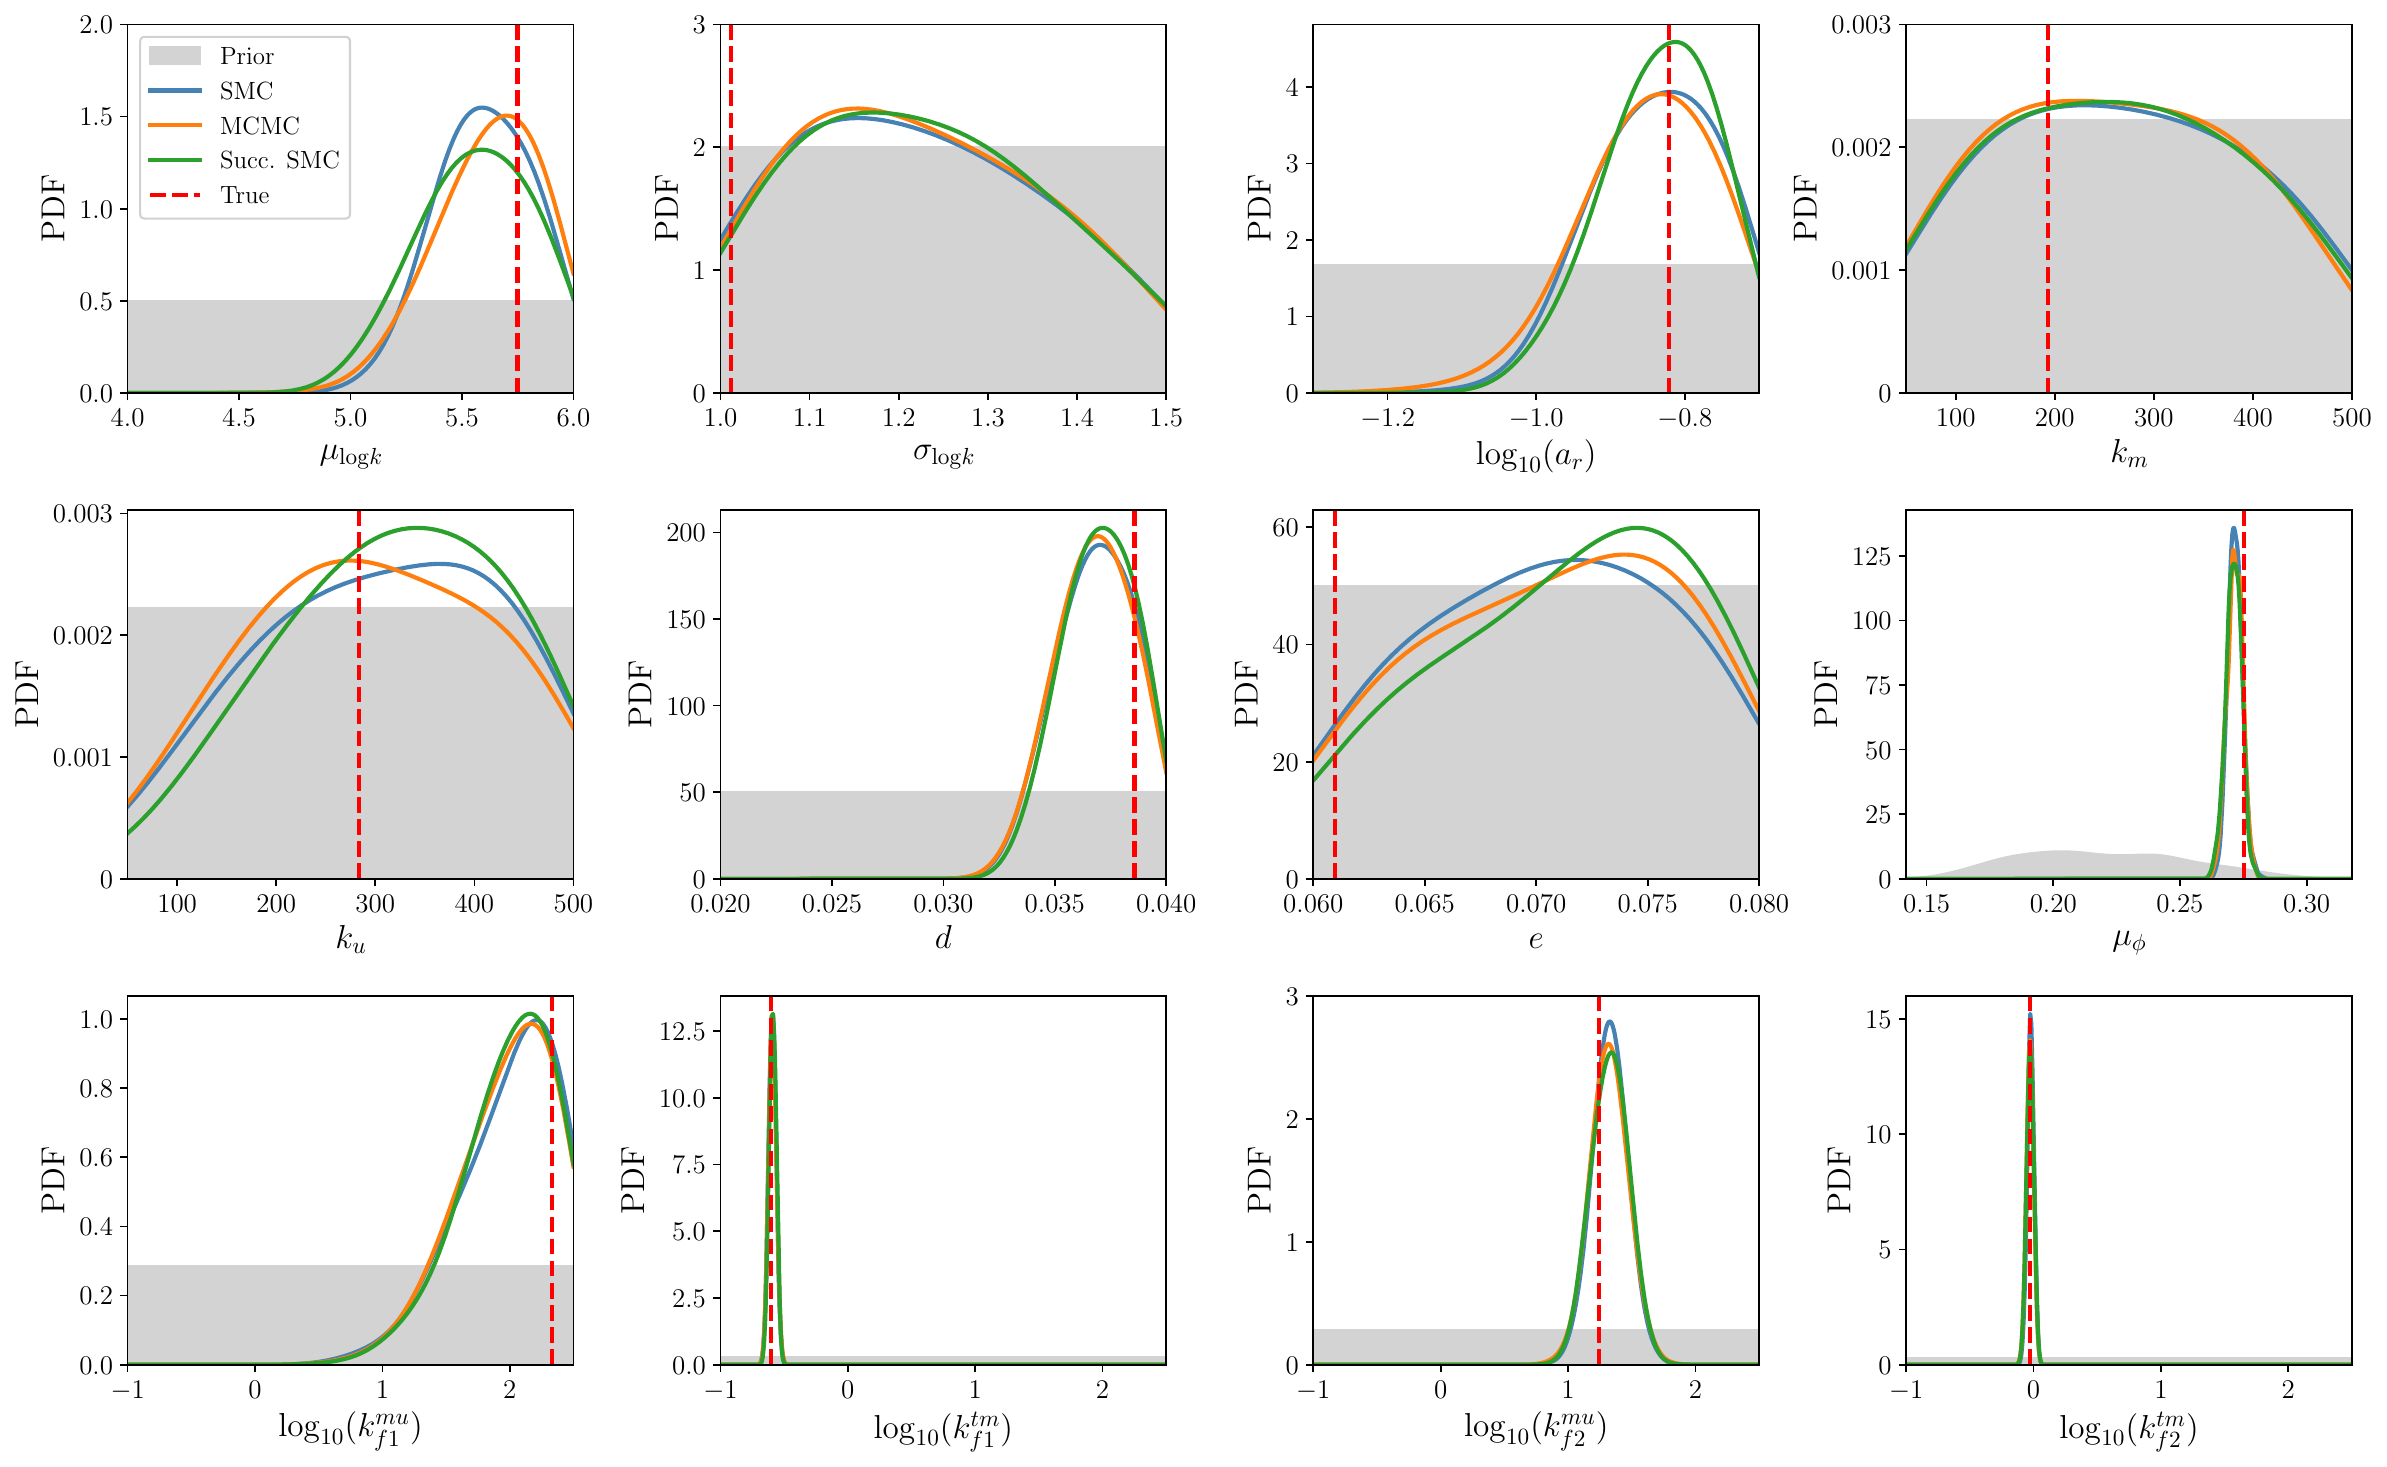}
\caption{Marginal posterior distributions of the 11 geological metaparameters and derived mean porosity $\mu_\phi$ for Case~1B. Results are shown for single-stage SMC (blue) and MCMC (orange) using observations through year~12, and for successive SMC (green), which uses observations through year~6 followed by additional observations at years~8, 10, and 12. The MCMC results are from the 50-hour run, which did not satisfy the less-stringent convergence criterion $\max_{j=1,\ldots,11}\widehat{R}_j<1.05$. Prior distributions are shown in gray, and the true values are indicated by the red dashed vertical lines.}
\label{fig:6t-s9-marg}
\end{figure}


Figs.~\ref{fig:317-rhat}--\ref{fig:317-wells-p} display results for Case~3. This case involves a different synthetic true model, which leads to qualitatively different CO$_2$ saturation fields and pressure distributions than were observed for Case~1. Fig.~\ref{fig:317-rhat} shows the MCMC convergence diagnostics, and Fig.~\ref{fig:317-marg} compares the marginal posterior metaparameter distributions obtained using SMC and MCMC. Figs.~\ref{fig:317-plumes} and~\ref{fig:317-pmap} show representative CO$_2$ saturation and pressure fields, while Figs.~\ref{fig:317-wells-sw} and~\ref{fig:317-wells-p} present the corresponding predictions at observation wells. The SMC and MCMC results are again in overall agreement and provide substantial reduction in predictive uncertainty relative to the prior.


\begin{figure}[!htbp]
\centering
\includegraphics[width=\linewidth]{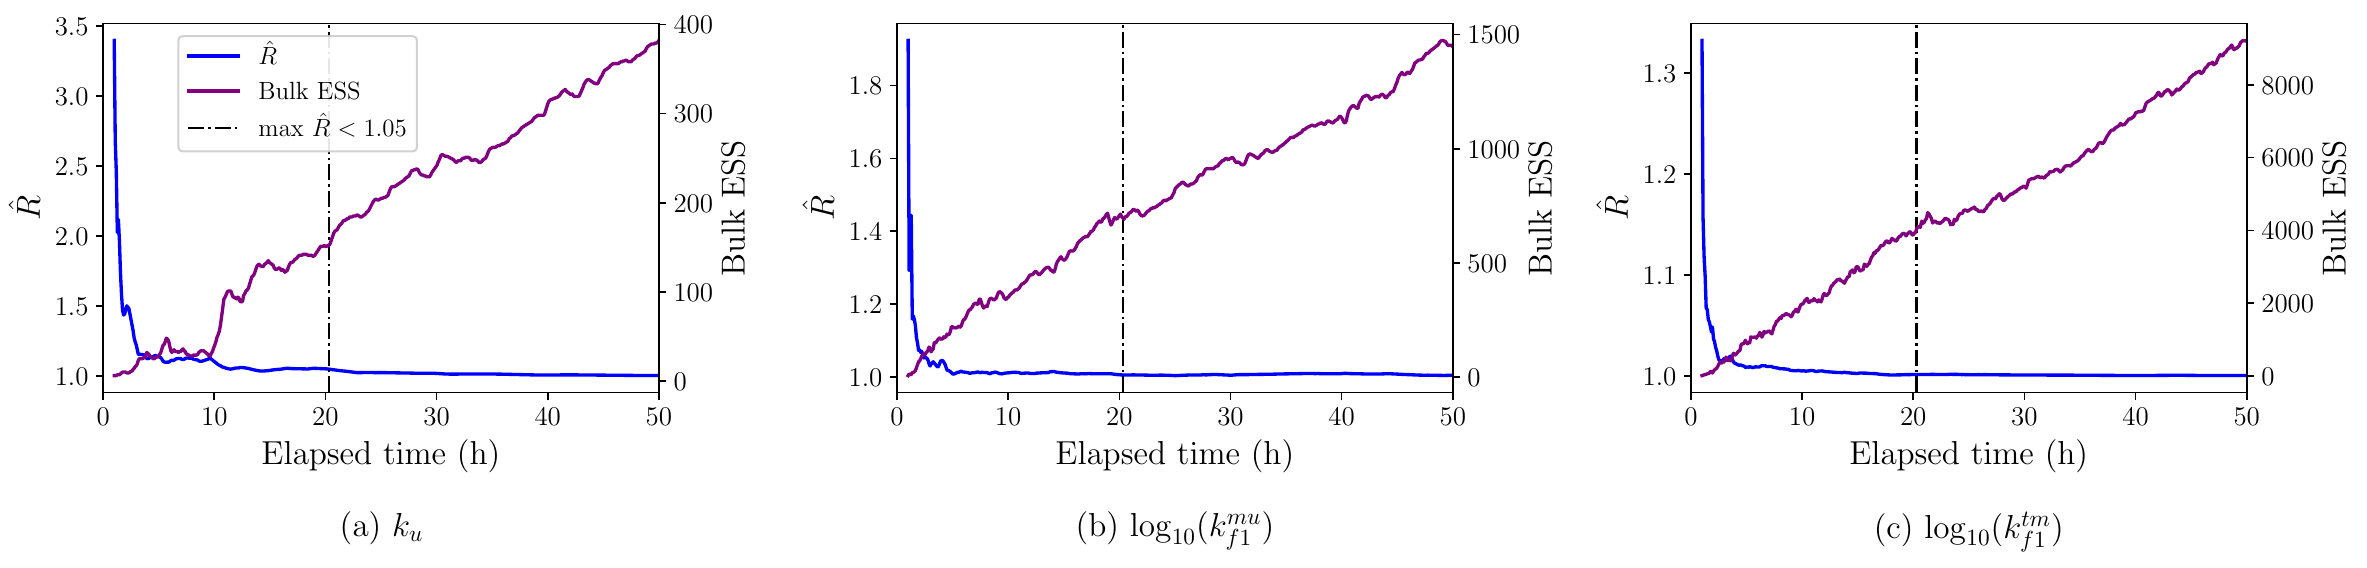}
\caption{MCMC convergence diagnostics for Case~3. The $\widehat{R}$ statistic (left axis) and bulk effective sample size (bulk ESS; right axis) are shown as functions of elapsed time for three metaparameters: (a)~$k_u$ (minimum bulk ESS), (b)~$\log_{10}(k_{f1}^{mu})$ (median bulk ESS), and (c)~$\log_{10}(k_{f1}^{tm})$ (maximum bulk ESS), based on the values at the end of the 50-hour run. The vertical dashed line at 20.3~hours indicates the satisfaction of the convergence criterion $\max_{j=1,\ldots,11}\widehat{R}_j<1.05$. The MCMC calculation terminates at 50~hours upon reaching the time limit specified in the stopping rule.}
\label{fig:317-rhat}
\end{figure}


\begin{figure}[!htbp]
\centering
\includegraphics[width=\linewidth]{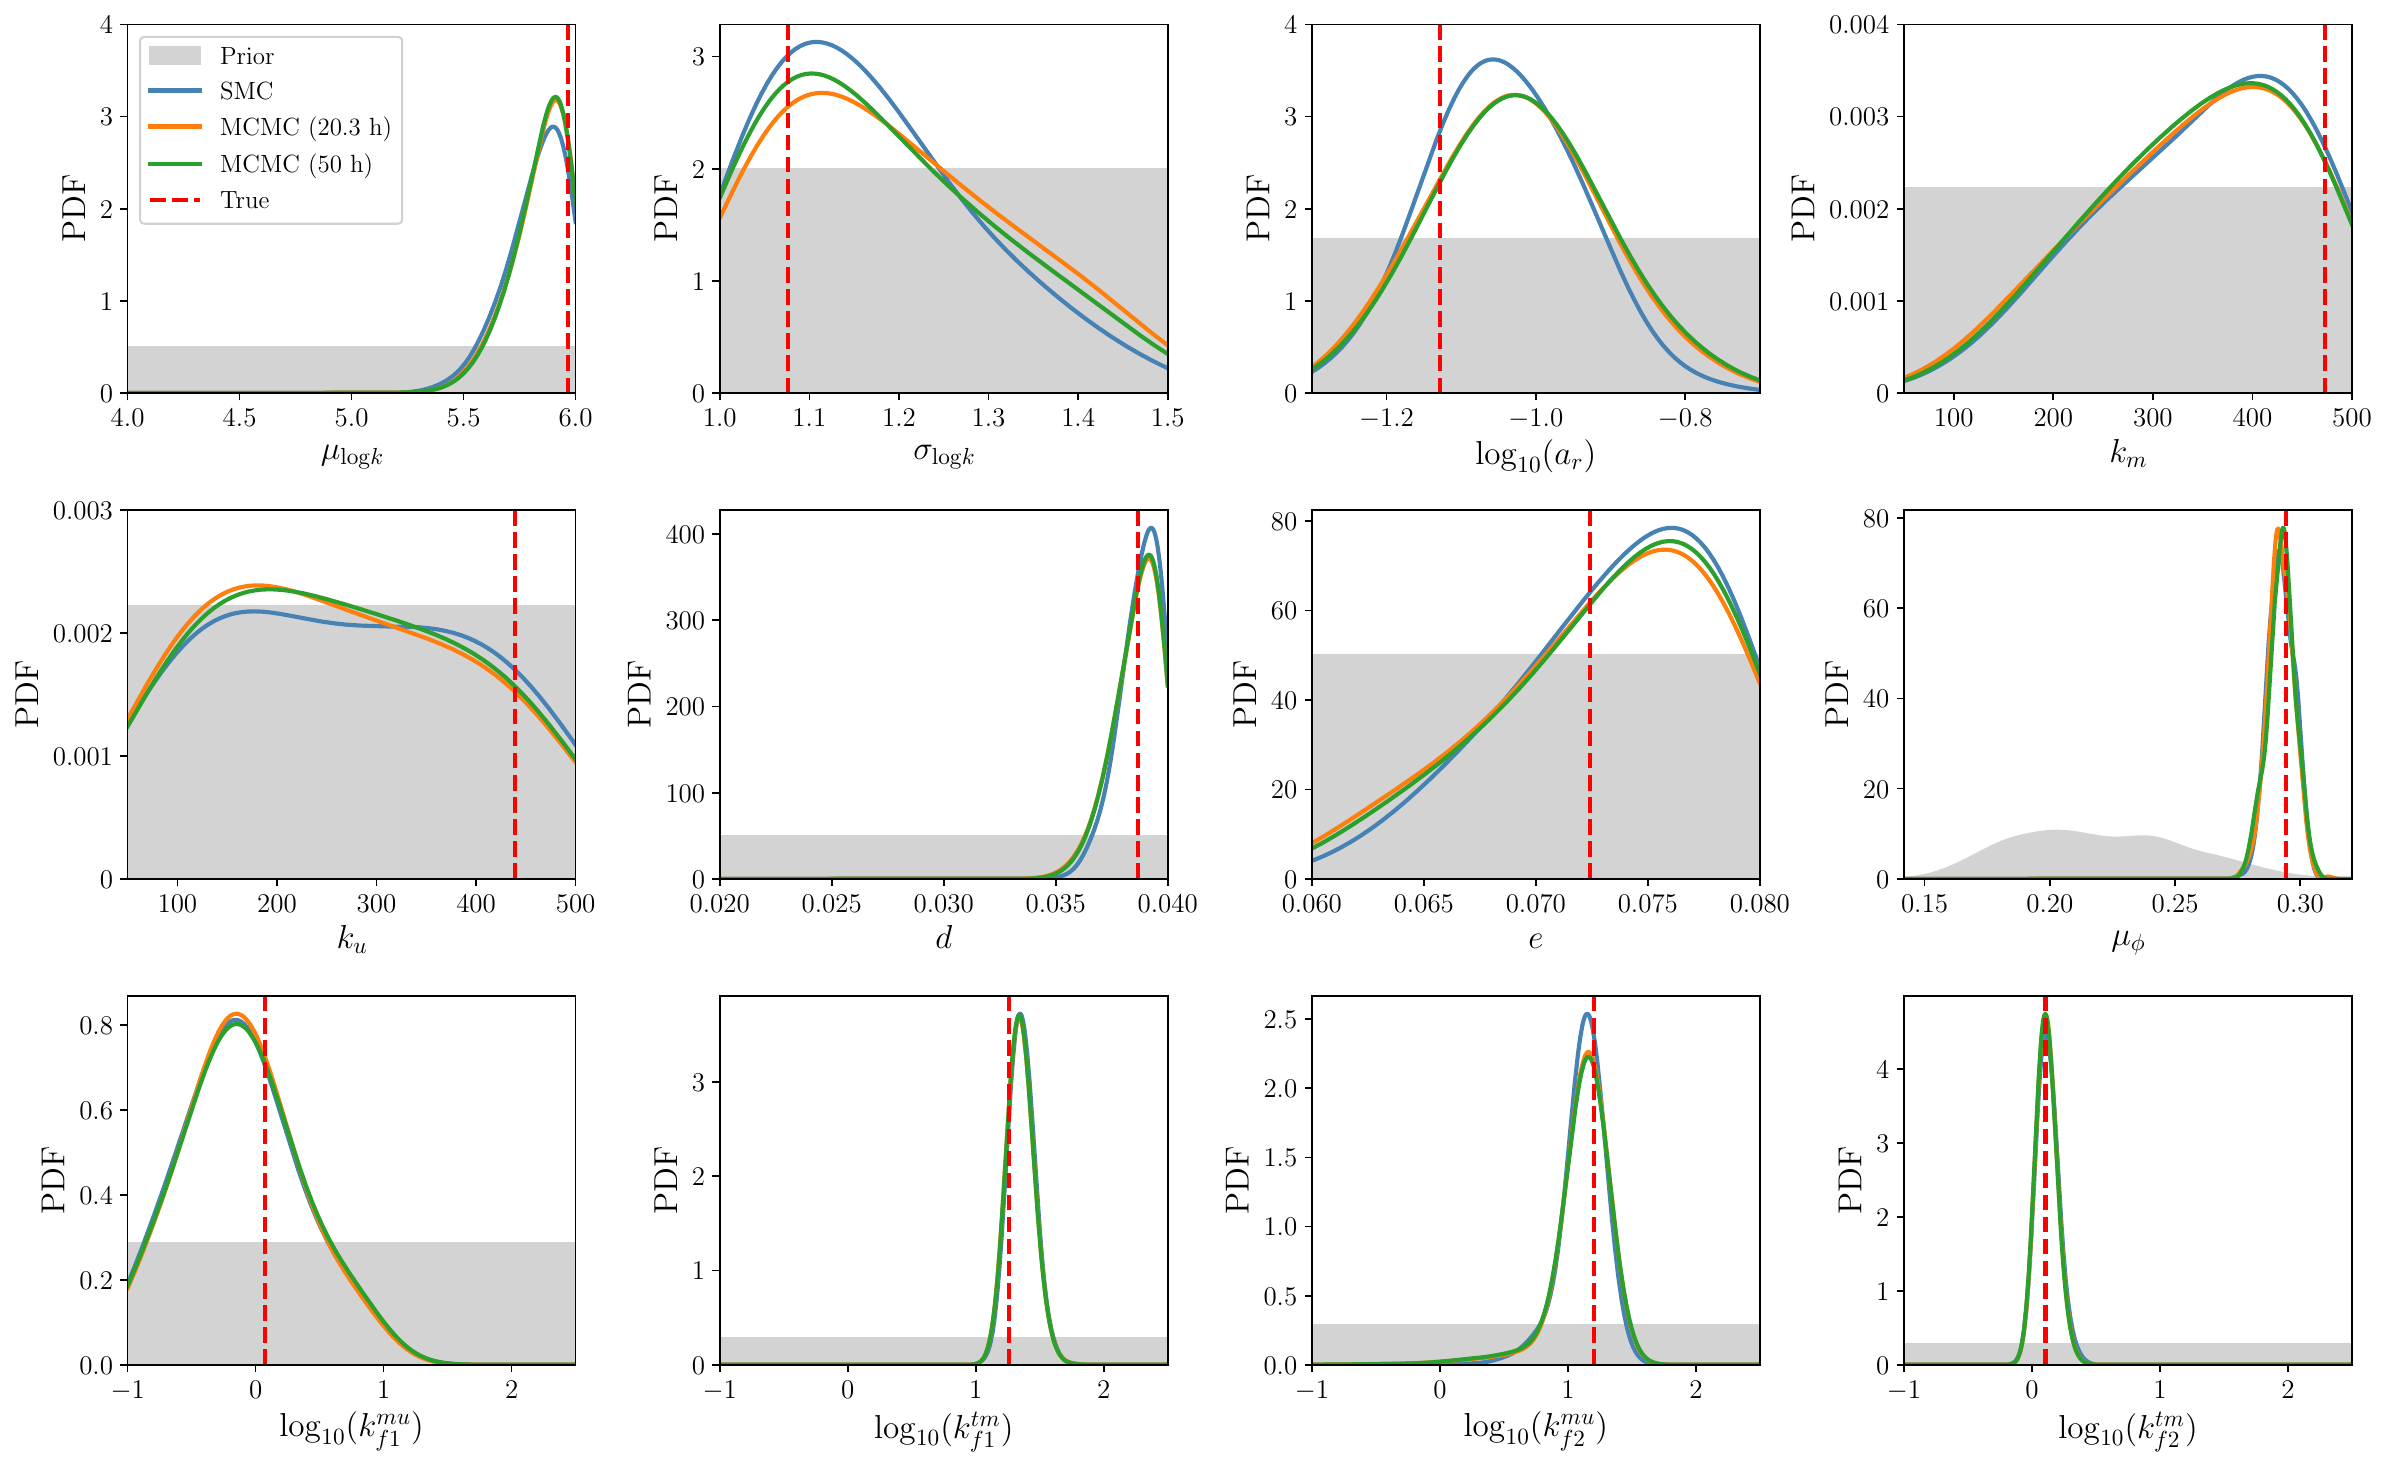}
\caption{Marginal posterior distributions of the 11 geological metaparameters and derived mean porosity $\mu_\phi$ for Case~3. Results are shown for SMC (blue), MCMC at the satisfaction of $\max_{j=1,\ldots,11}\widehat{R}_j<1.05$ (20.3~hours, orange), and MCMC at the end of the 50-hour run (green). Prior distributions are shown in gray, and the true values are indicated by the red dashed vertical lines.}
\label{fig:317-marg}
\end{figure}


\begin{centeredfigurepage}
\includegraphics[width=\linewidth]{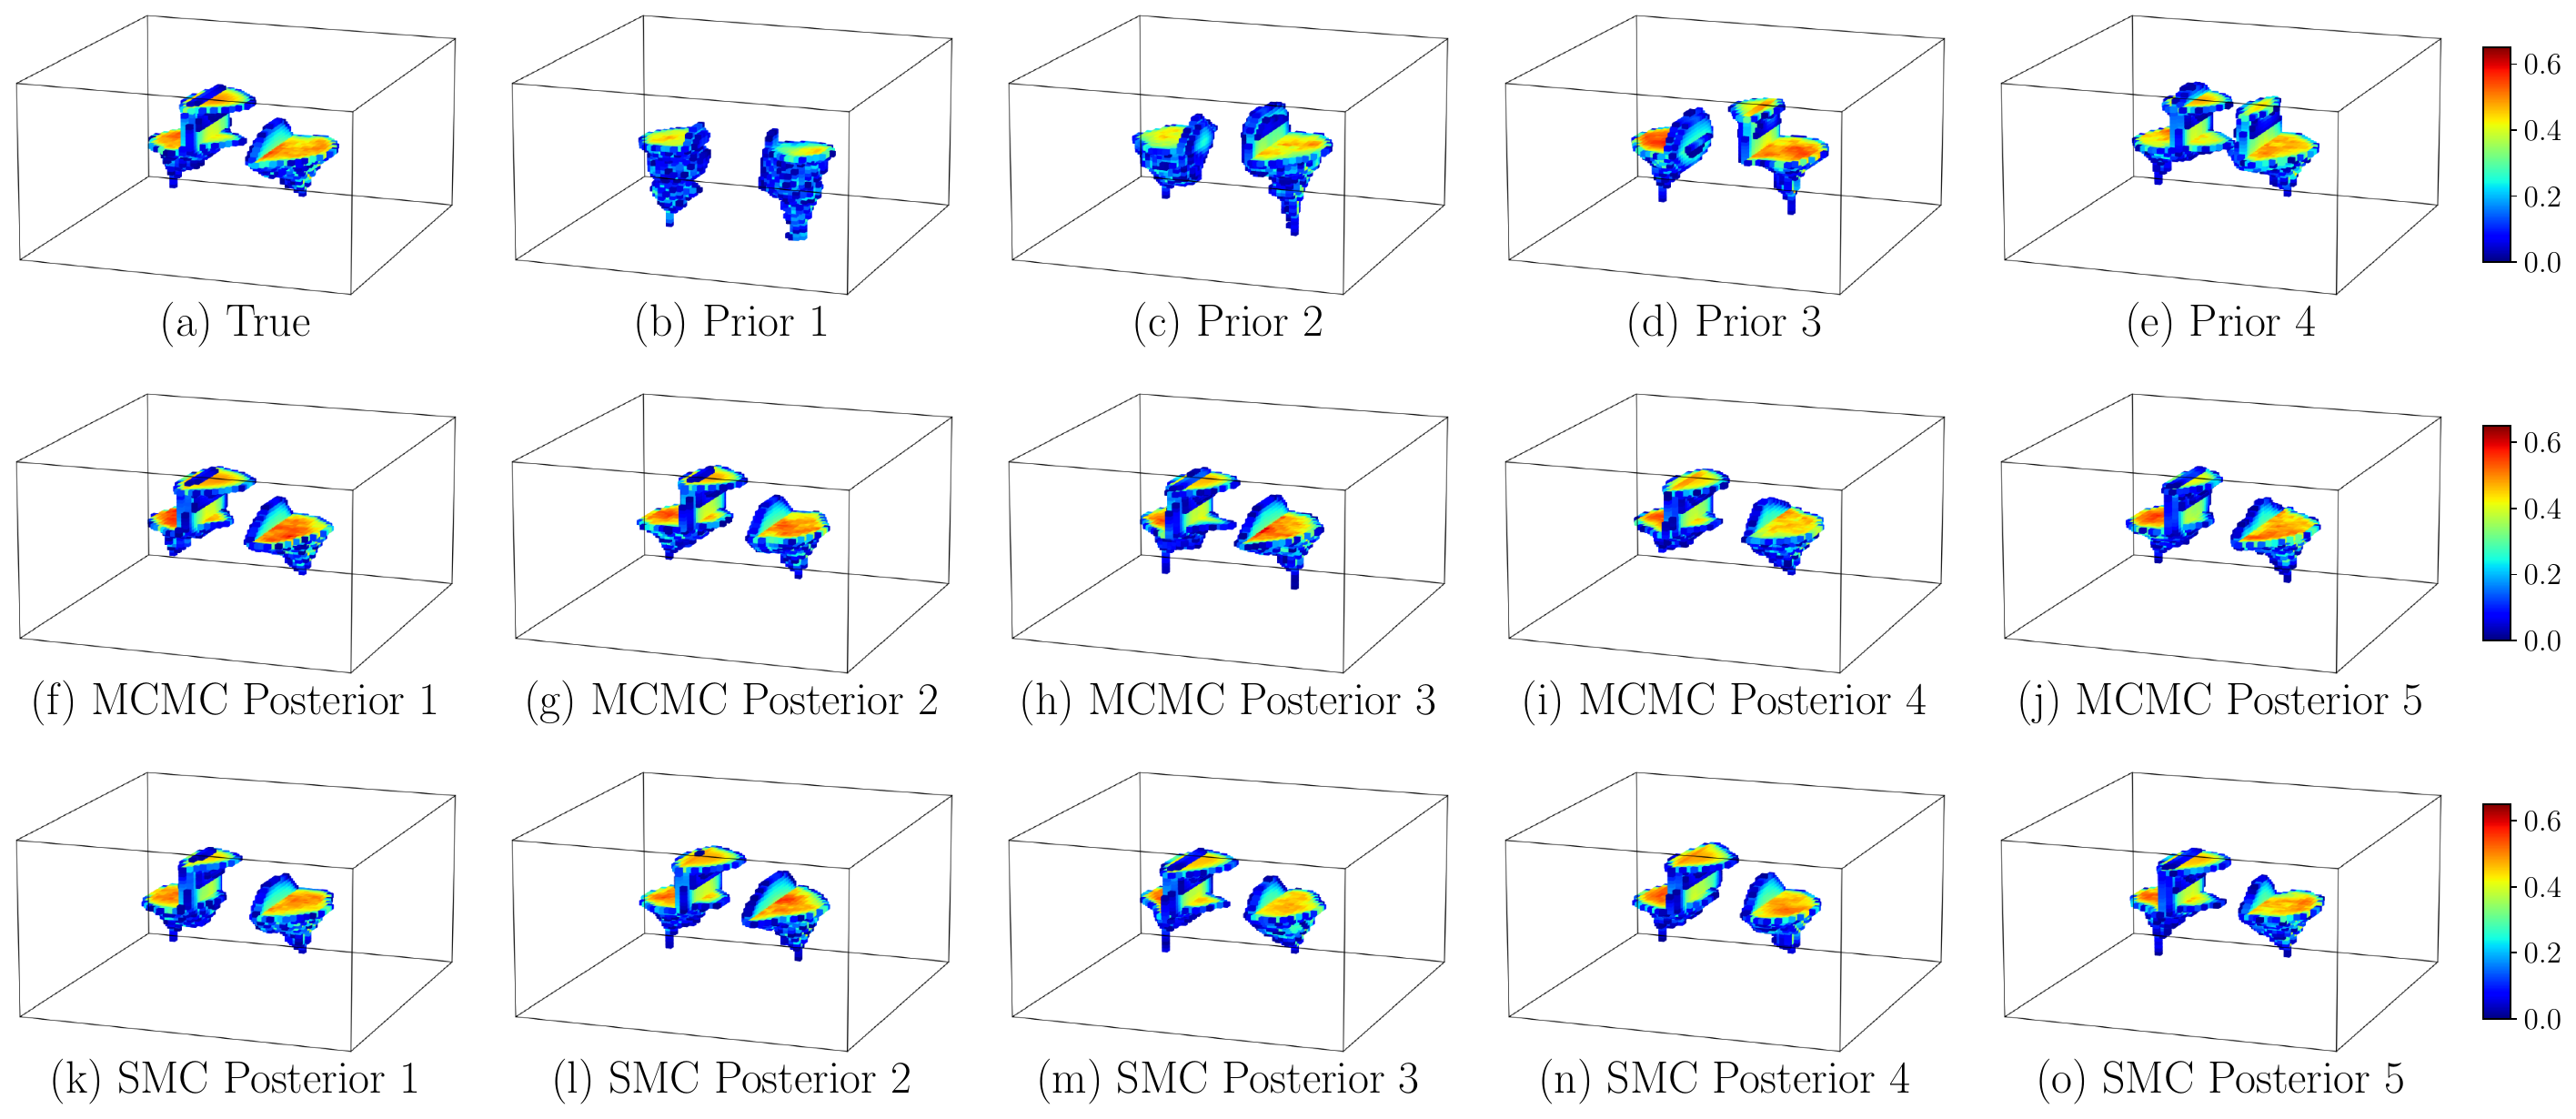}
\caption{Representative 3D CO$_2$ saturation plumes at 50~years for Case~3. Top row shows the true model and four representative prior realizations, and middle and bottom rows show representative MCMC and SMC posterior samples. Compared to the prior plumes, both sets of posterior results show less variability and general agreement with the true plume geometry.}
\label{fig:317-plumes}
\end{centeredfigurepage}


\begin{figure}[!htbp]
\centering
\includegraphics[width=0.95\linewidth]{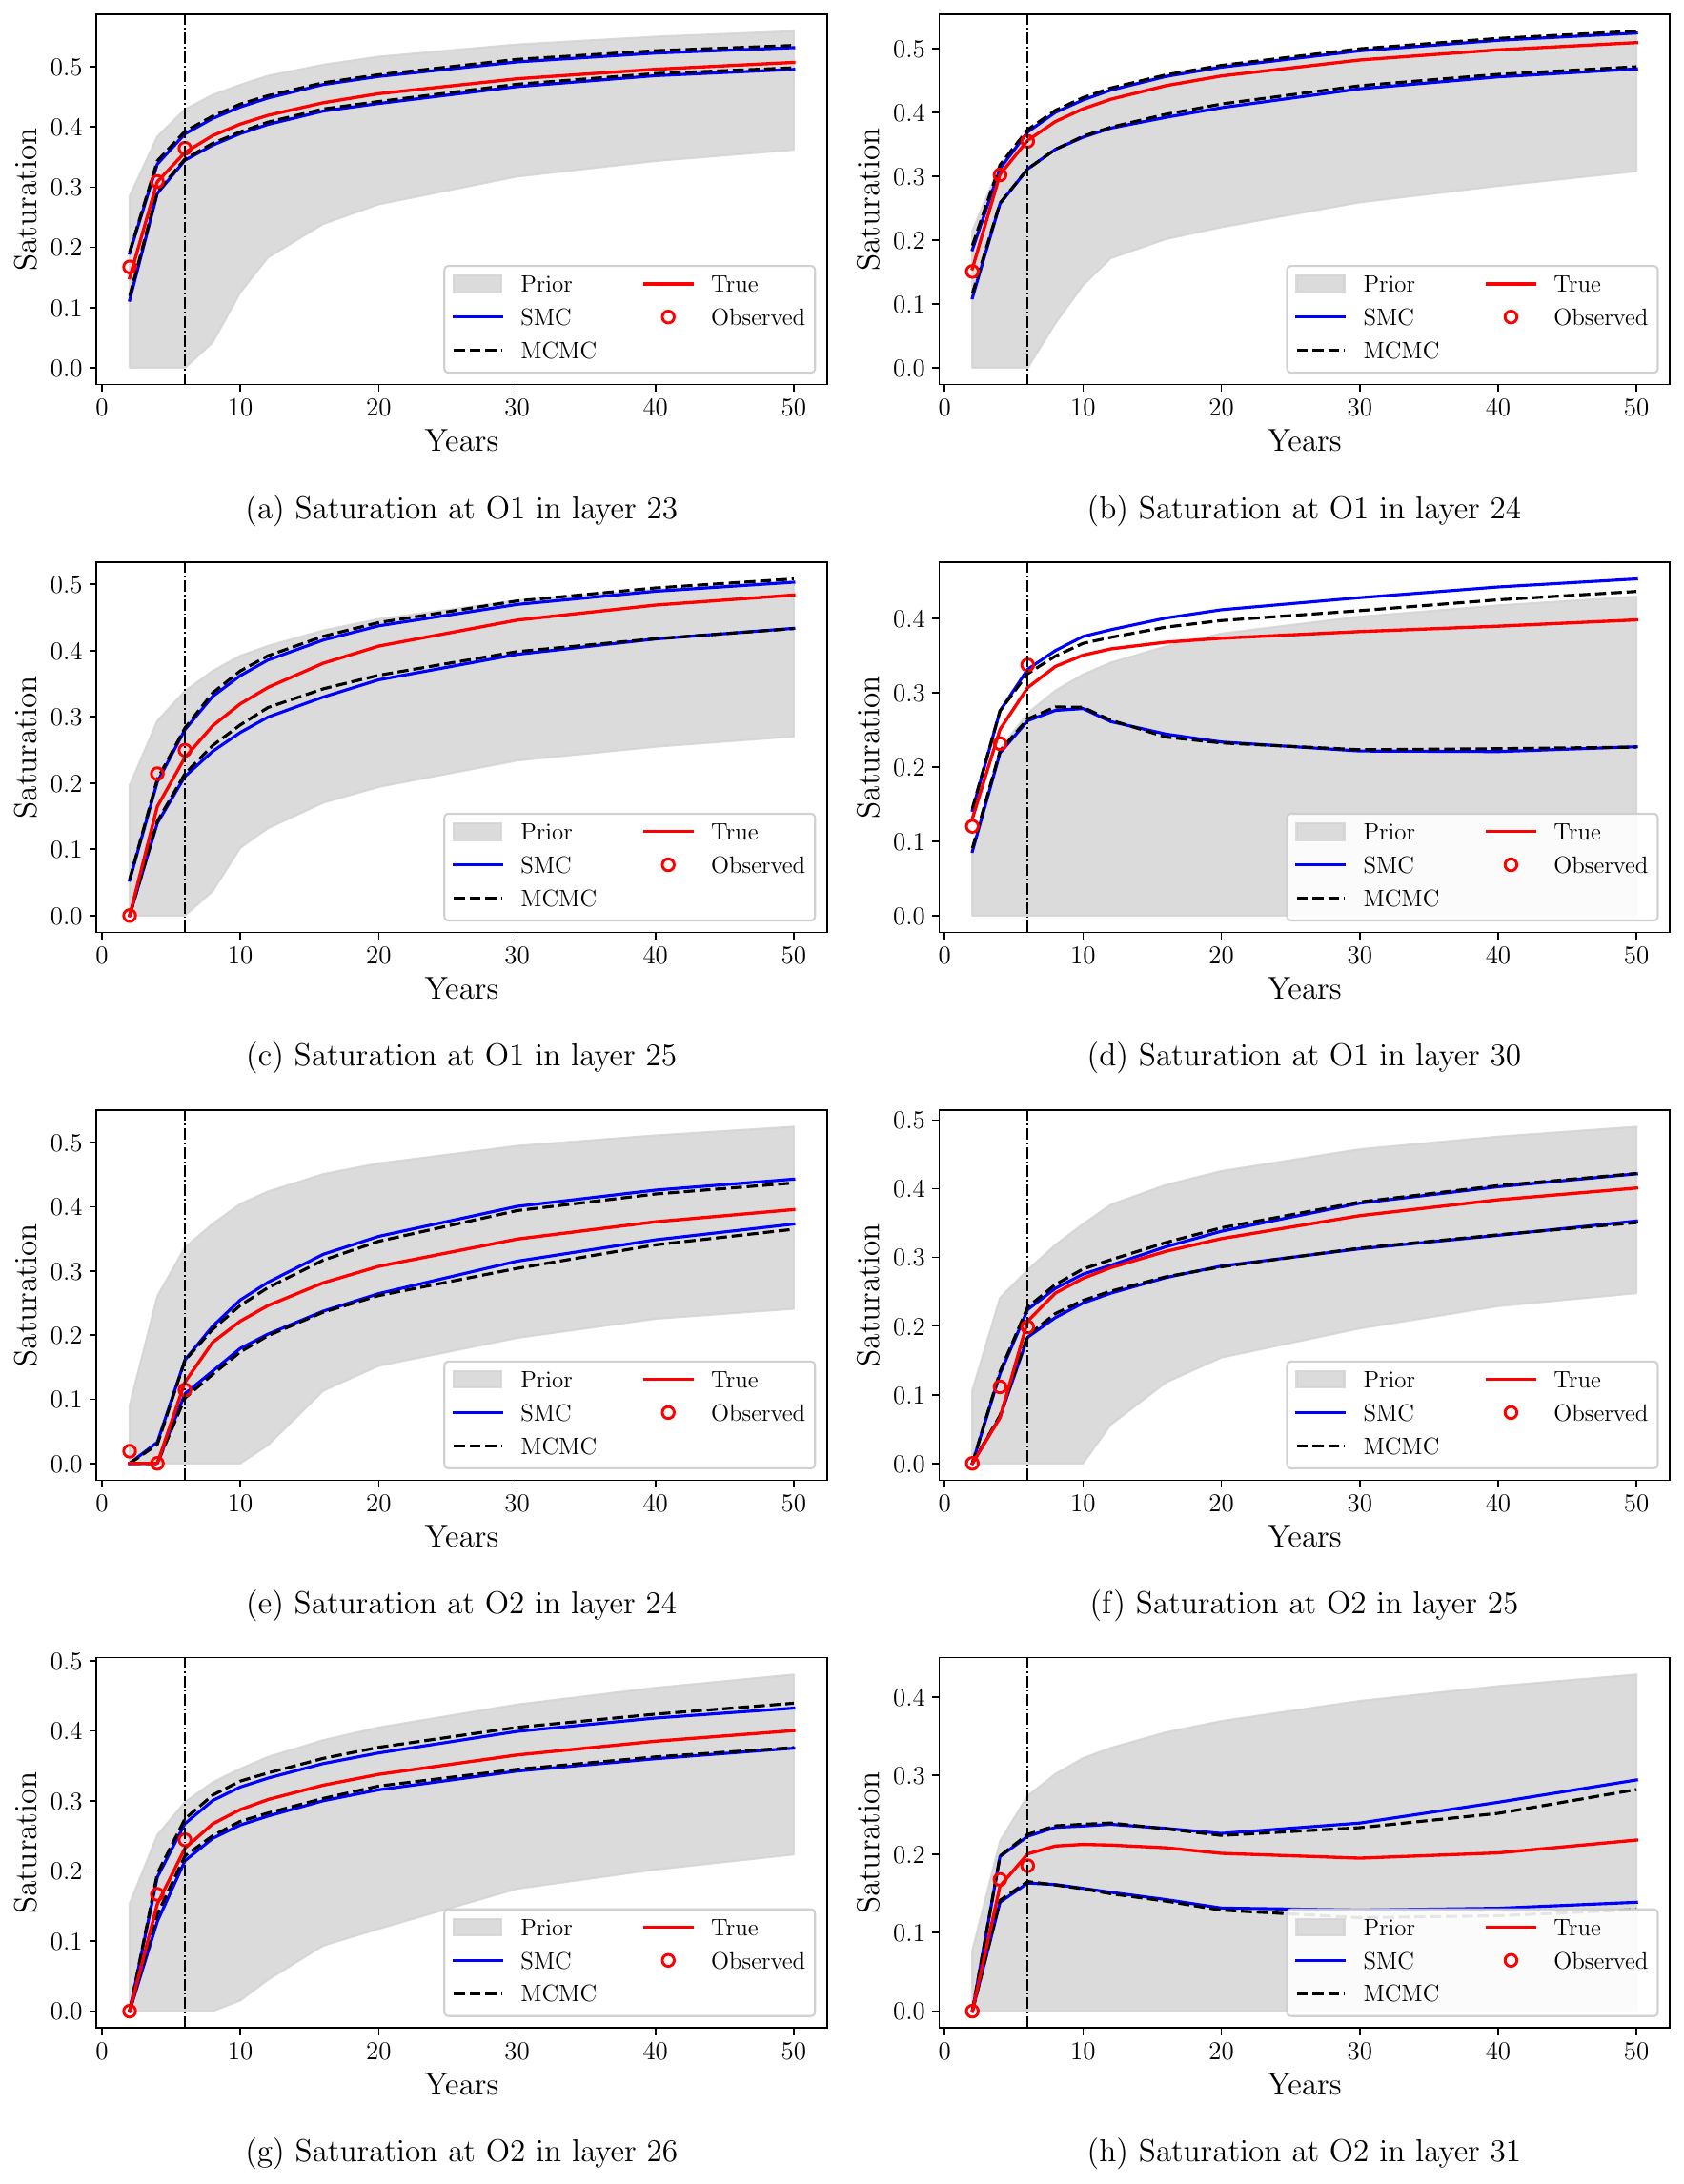}
\caption{Posterior $\mathrm{P}_{10}$--$\mathrm{P}_{90}$ predictions of CO$_2$ saturation at observation wells O1 and O2 in various layers for Case~3. Results are shown for SMC (blue) and MCMC (black dashed), along with the prior $\mathrm{P}_{10}$--$\mathrm{P}_{90}$ range (gray), true response (red), and observed data (red circles). Vertical dashed line indicates the end of the data assimilation time window at 6~years.}
\label{fig:317-wells-sw}
\end{figure}


\begin{figure}[!htbp]
\centering
\includegraphics[width=\linewidth]{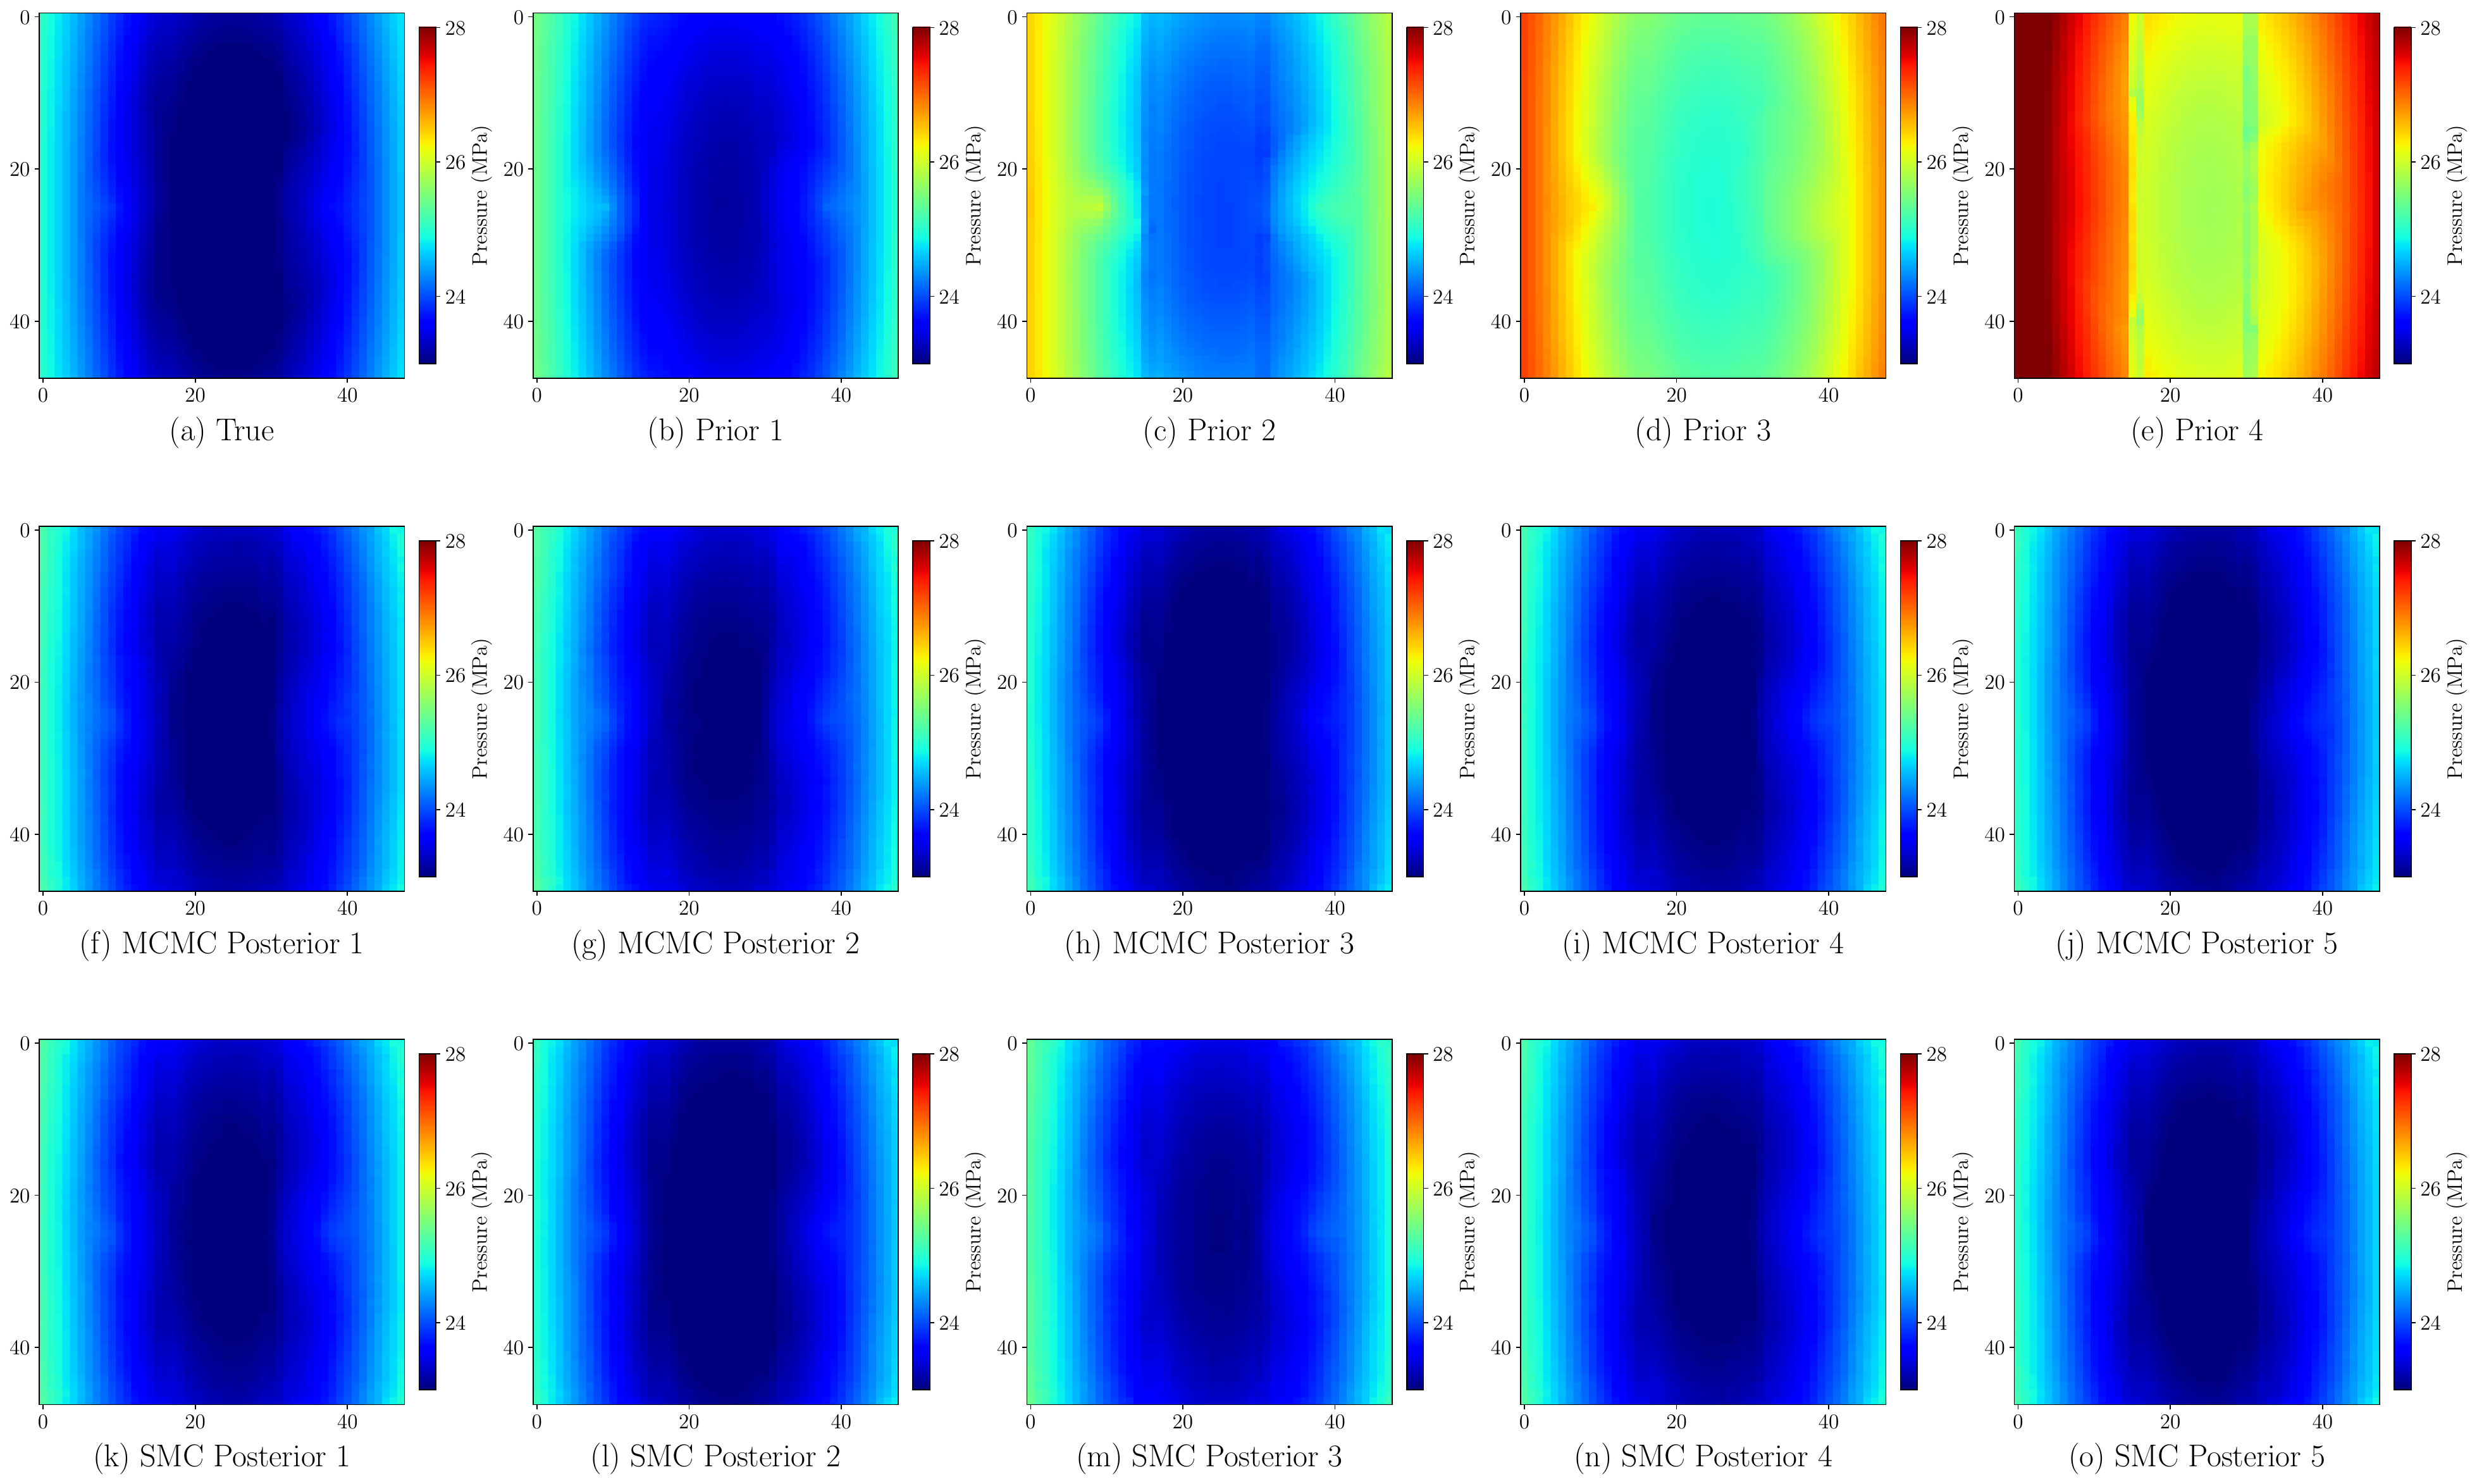}
\caption{Pressure maps in the uppermost layer of the storage aquifer at 50~years for Case~3. Top row shows the true model and four representative prior realizations, and the middle and bottom rows show representative MCMC and SMC posterior samples.}
\label{fig:317-pmap}
\end{figure}


\begin{figure}[!htbp]
\centering
\includegraphics[width=0.85\linewidth]{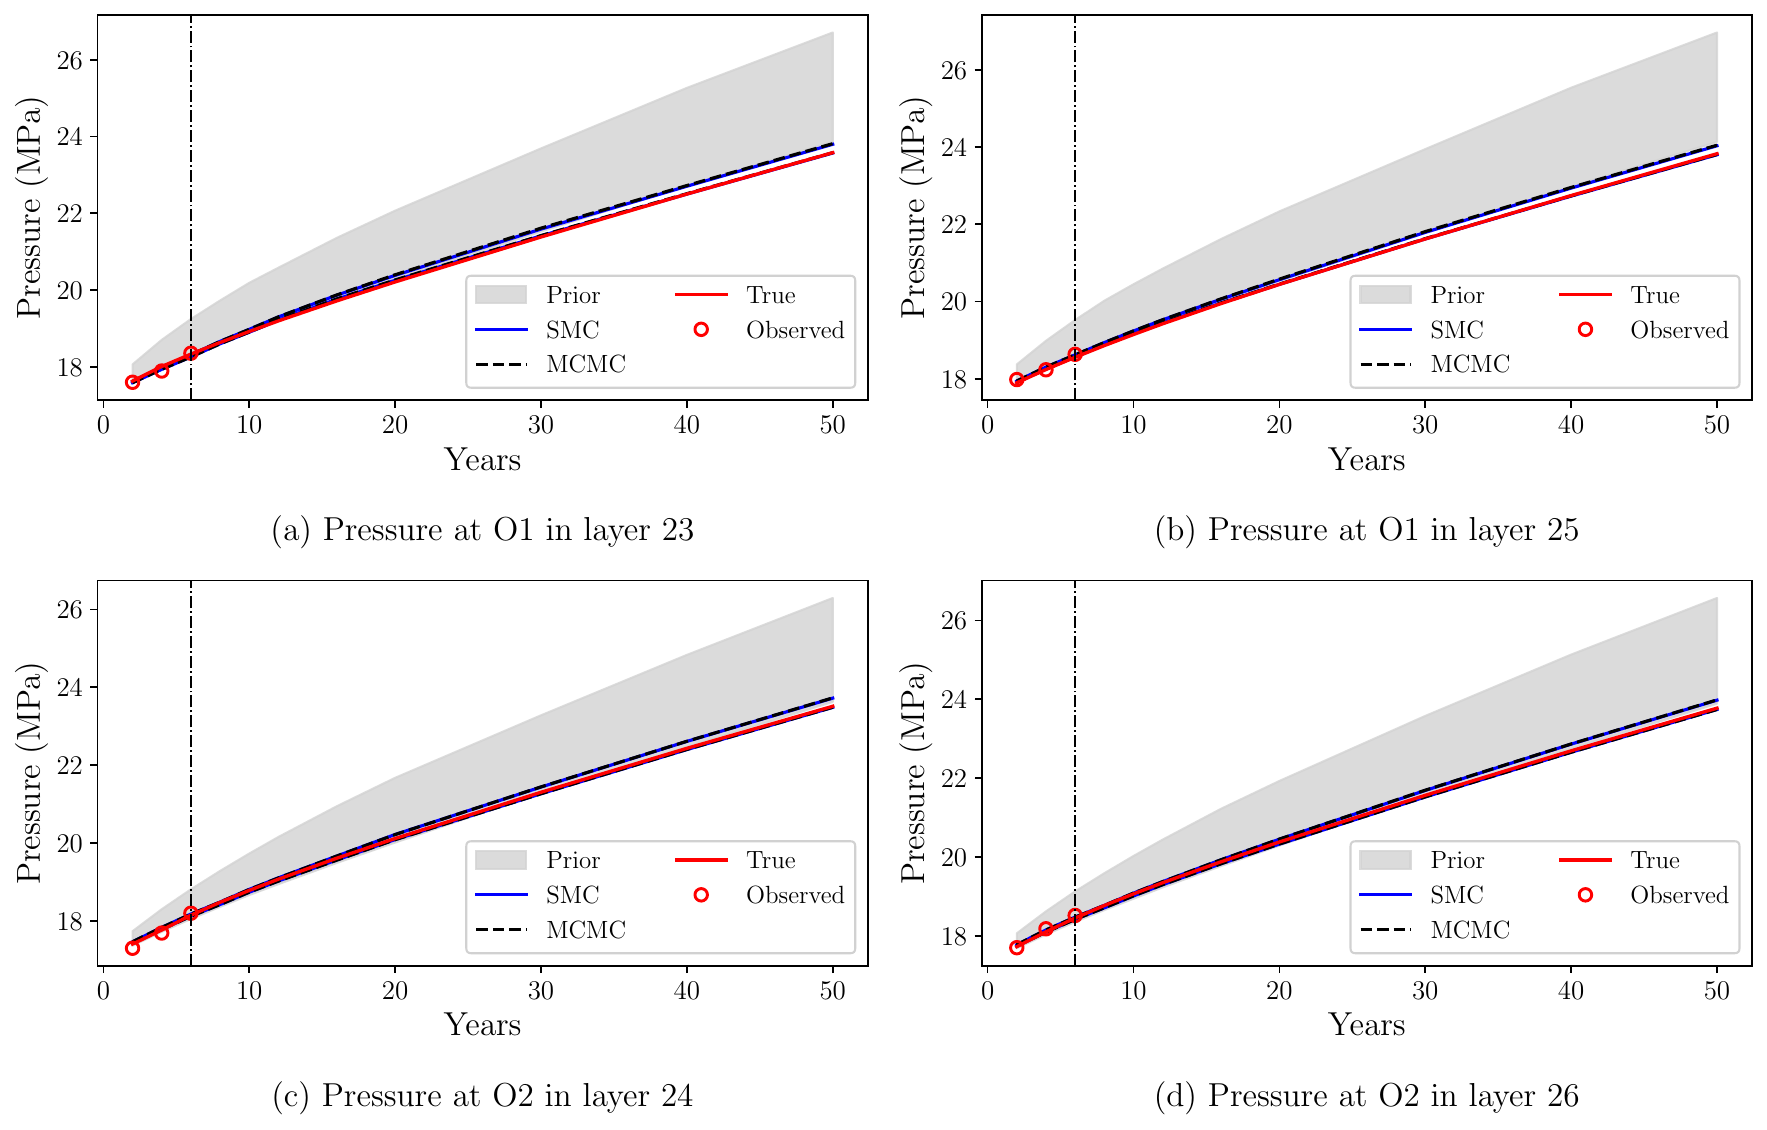}
\caption{Posterior $\mathrm{P}_{10}$--$\mathrm{P}_{90}$ predictions of pressure at observation wells O1 and O2 in various layers for Case~3. Results are shown for SMC (blue) and MCMC (black dashed), along with the prior $\mathrm{P}_{10}$--$\mathrm{P}_{90}$ range (gray), true response (red), and observed data (red circles). Vertical dashed line indicates the end of the data assimilation time window at 6~years.}
\label{fig:317-wells-p}
\end{figure}


\FloatBarrier


\section{Additional results for the channelized oil-water system}
\label{sec:case-4}

In Section~6 of the main paper, we presented well-level injection and production rates for Case~2. Field-level rate predictions for this case are provided in Fig.~\ref{fig:tm411-field-rates}, where we again observe close agreement between the two methods and large reductions in prior uncertainty.


\begin{figure}[!htbp]
\centering
\includegraphics[width=1.0\linewidth]{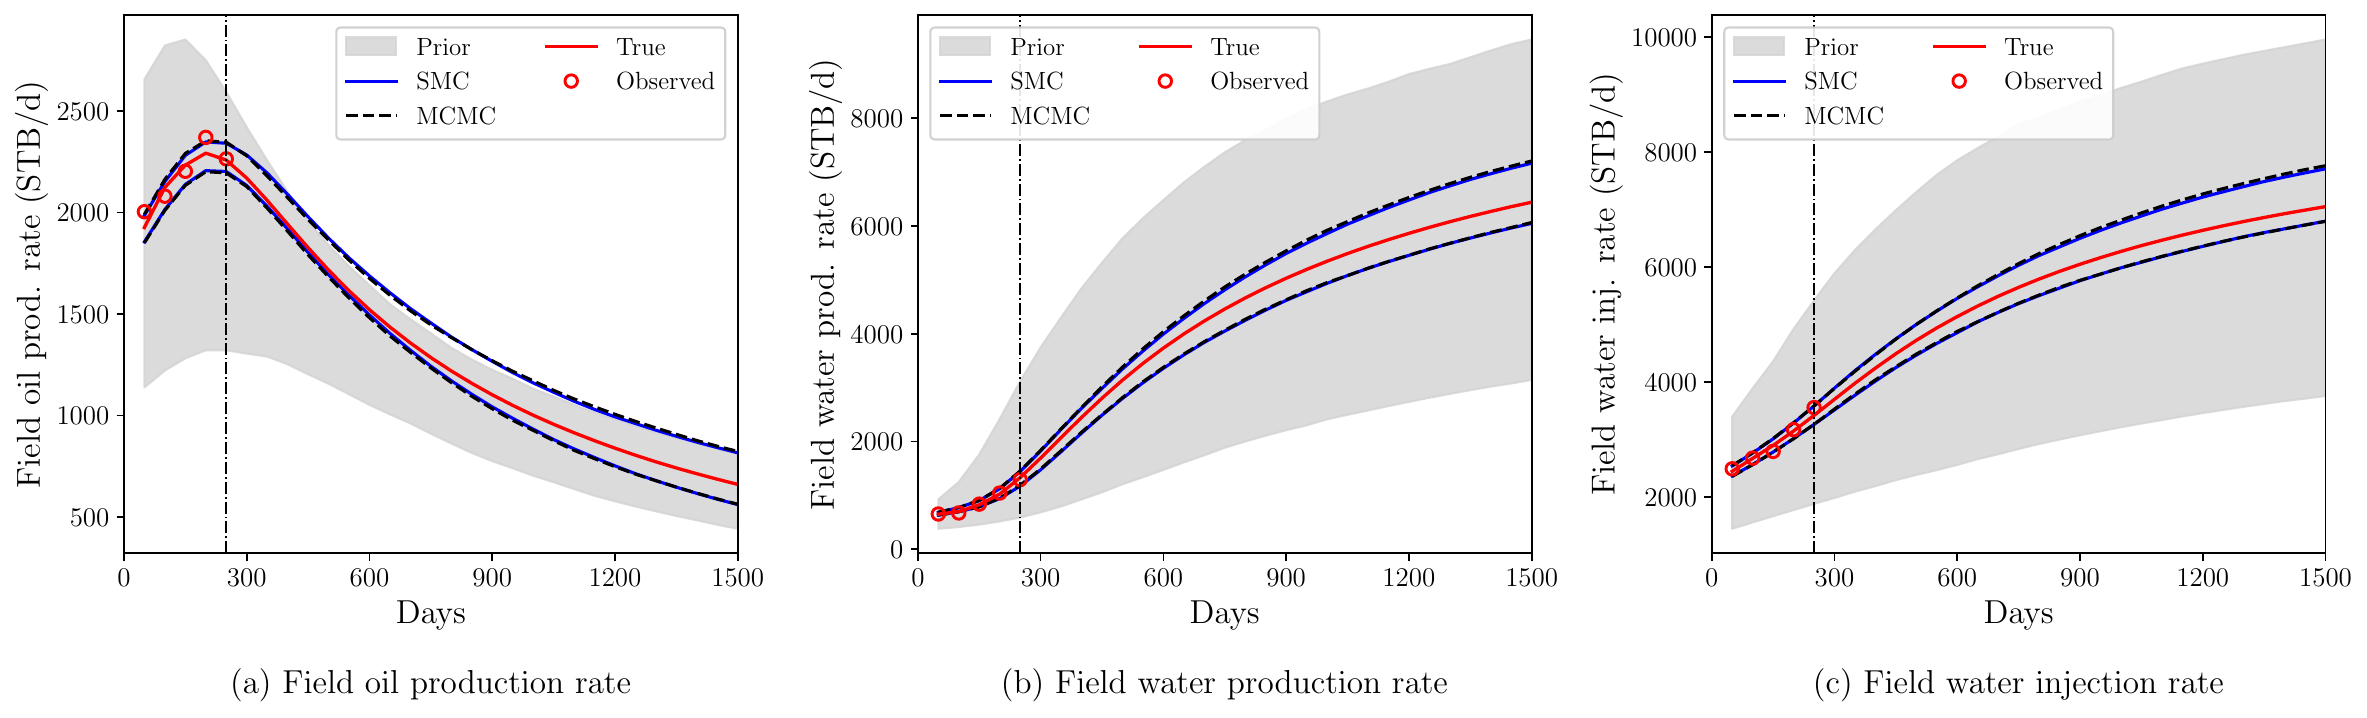}
\caption{Posterior $\mathrm{P}_{10}$--$\mathrm{P}_{90}$ predictions of field rates in Case~2. SMC and MCMC results are shown in blue and black dashed lines, respectively, while the gray regions denote the prior $\mathrm{P}_{10}$--$\mathrm{P}_{90}$ ranges. Red curves represent the true data, and red circles indicate the observed data. The vertical black dashed line marks the end of the data assimilation time window at 250~days.}
\label{fig:tm411-field-rates}
\end{figure}


Figs.~\ref{fig:tm104-rhat-ess}--\ref{fig:tm104-field-rates} present results for Case~4. This case involves a synthetic true model with a smaller average channel width and a larger mud fraction than Case~2. Fig.~\ref{fig:tm104-rhat-ess} shows the MCMC convergence diagnostics, and Figs.~\ref{fig:tm104-k-phi-marginals} and~\ref{fig:tm104-scenario-marginals} compare the marginal posterior distributions of the petrophysical and geometric metaparameters. Fig.~\ref{fig:tm104-facies-geomodels} displays representative facies geomodels, while Figs.~\ref{fig:tm104-well-rates} and~\ref{fig:tm104-field-rates} present the corresponding well and field-level rate predictions. The SMC and MCMC results continue to correspond closely in all quantities considered.


\begin{figure}[!htbp]
\centering
\includegraphics[width=1.0\linewidth]
{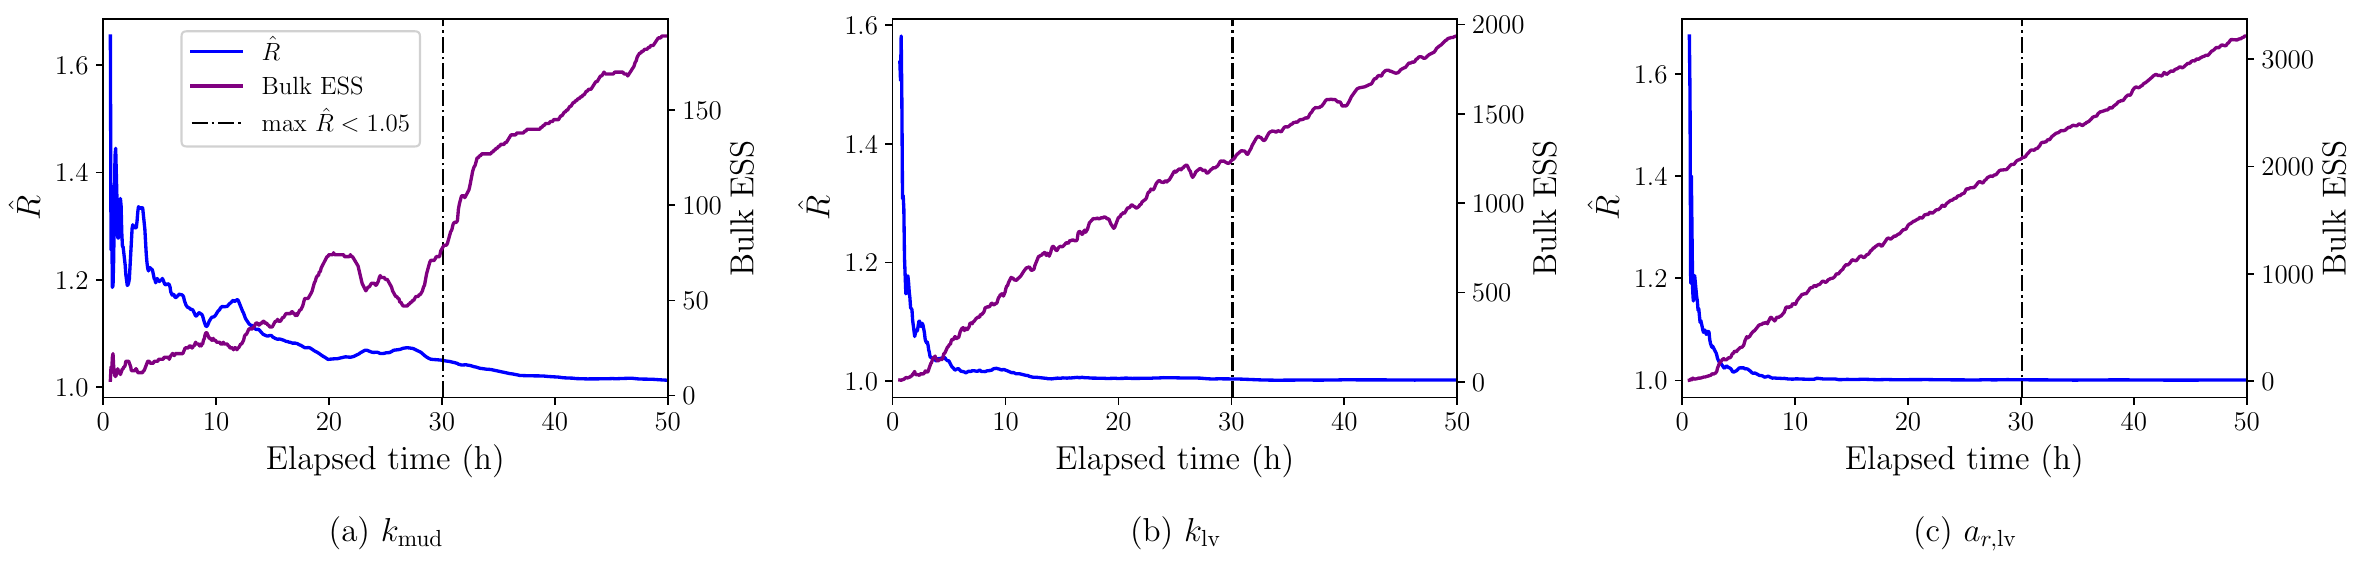}
\caption{MCMC convergence diagnostics for Case~4. The $\widehat{R}$ statistic (left axis) and bulk effective sample size (bulk ESS; right axis) are shown as functions of elapsed time for three metaparameters: (a)~$k_{\mathrm{mud}}$ (minimum bulk ESS), (b)~$k_{\mathrm{lv}}$ (median bulk ESS), and (c)~$a_{r,\mathrm{lv}}$ (maximum bulk ESS), based on the values at the end of the 50-hour run. The vertical dashed line at 30.1~hours indicates satisfaction of the convergence criterion $\max_{j=1,\ldots,9}\widehat{R}_j<1.05$. The MCMC calculation terminates at the 50-hour time limit without satisfying the more stringent criterion $\max_{j=1,\ldots,9}\widehat{R}_j<1.01$.}
\label{fig:tm104-rhat-ess}
\end{figure}


\begin{figure}[!htbp]
\centering
\includegraphics[width=0.95\linewidth]{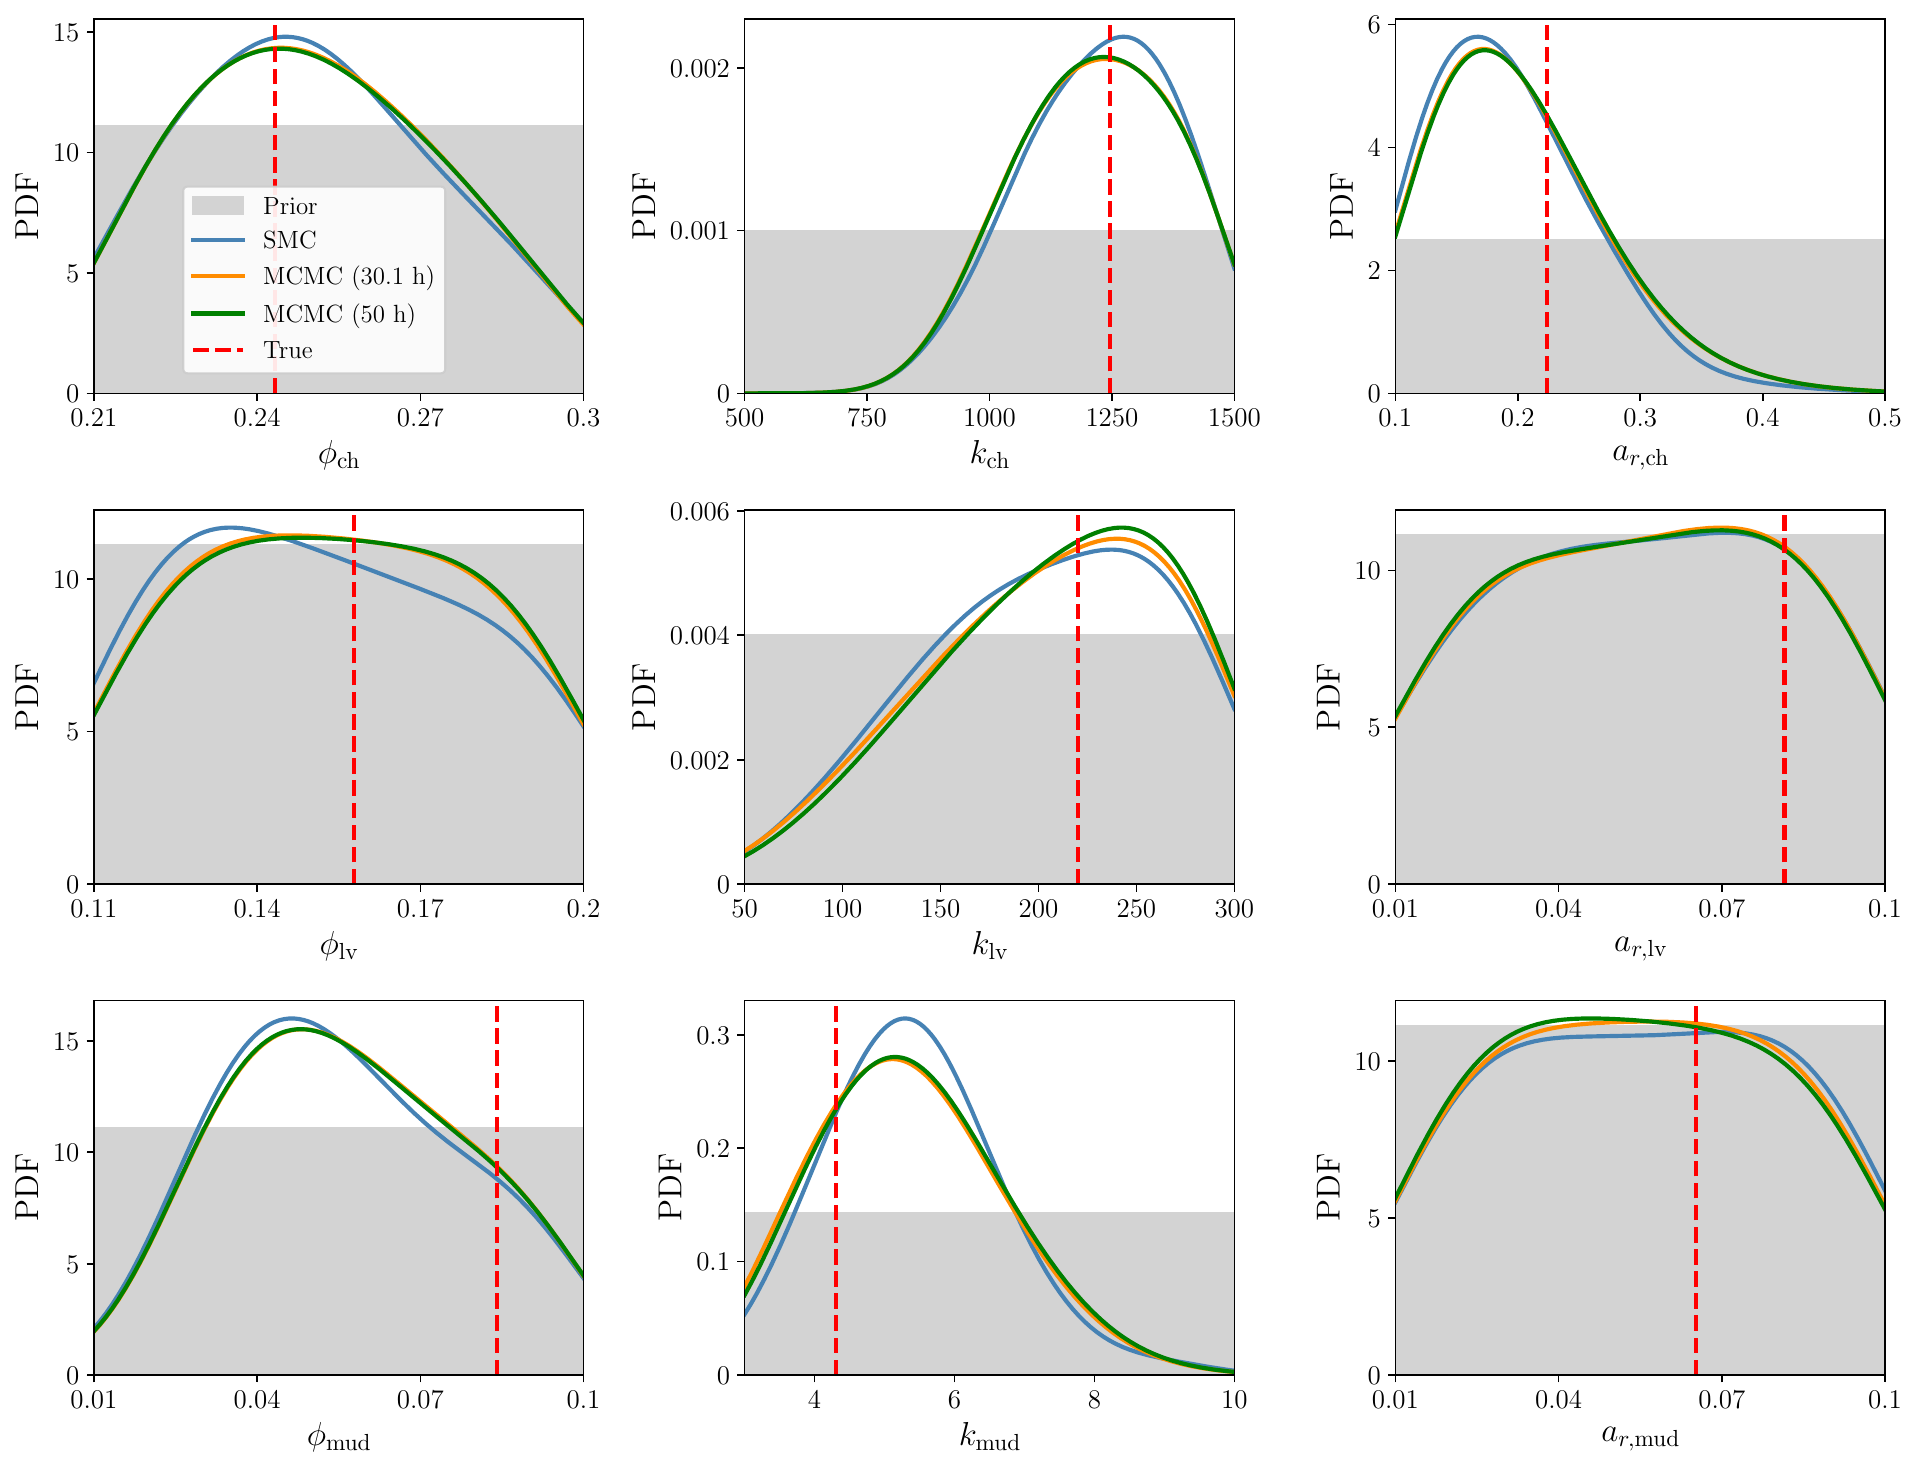}
\caption{Marginal posterior distributions of the nine facies-dependent petrophysical metaparameters in Case~4: porosity $\phi$, permeability $k$, and anisotropy ratio $a_r$ for the channel (top row), levee (middle row), and mud (bottom row) facies. Posterior distributions obtained with SMC are shown in blue. The MCMC distributions at the convergence criterion $\max_{j=1,\ldots,9}\widehat{R}_j<1.05$ (30.1~hours) and at the 50-hour time limit are shown in orange and green, respectively. Gray regions denote the uniform priors, and the red dashed vertical lines indicate the true parameter values.}
\label{fig:tm104-k-phi-marginals}
\end{figure}


\begin{figure}[!htbp]
\centering
\includegraphics[width=0.95\linewidth]{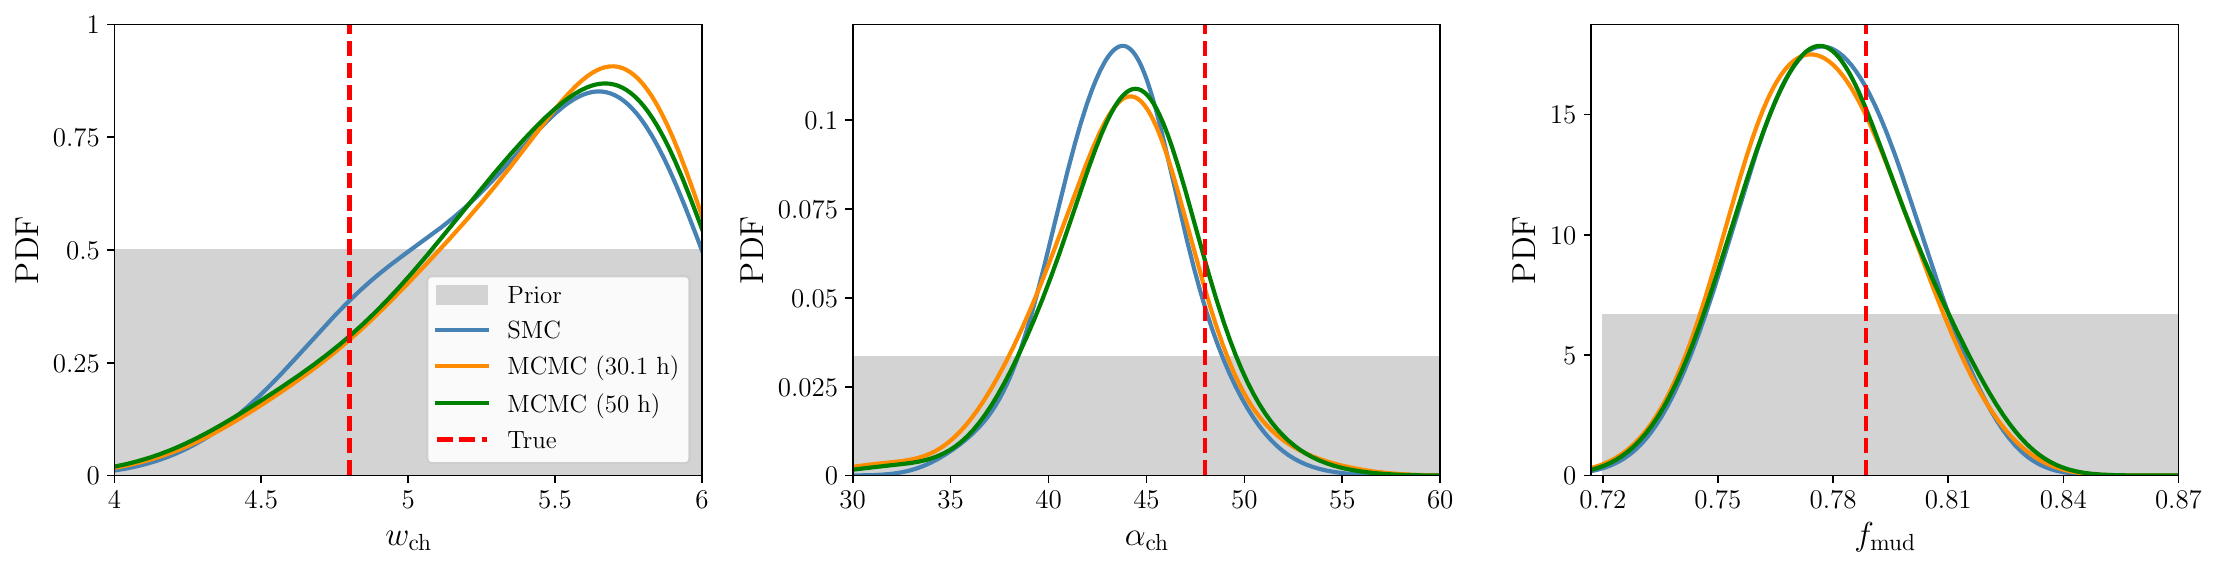}
\caption{Marginal posterior distributions of the three geometric metaparameters for Case~4, derived from the posterior facies realizations. Results are shown for SMC (blue), MCMC at the satisfaction of $\max_{j=1,\ldots,9}\widehat{R}_j<1.05$ (30.1~hours, orange), and MCMC at the 50-hour time limit (green). Gray regions indicate the uniform priors, and the red dashed vertical lines denote the true values.}
\label{fig:tm104-scenario-marginals}
\end{figure}


\begin{centeredfigurepage}
\includegraphics[width=\linewidth]{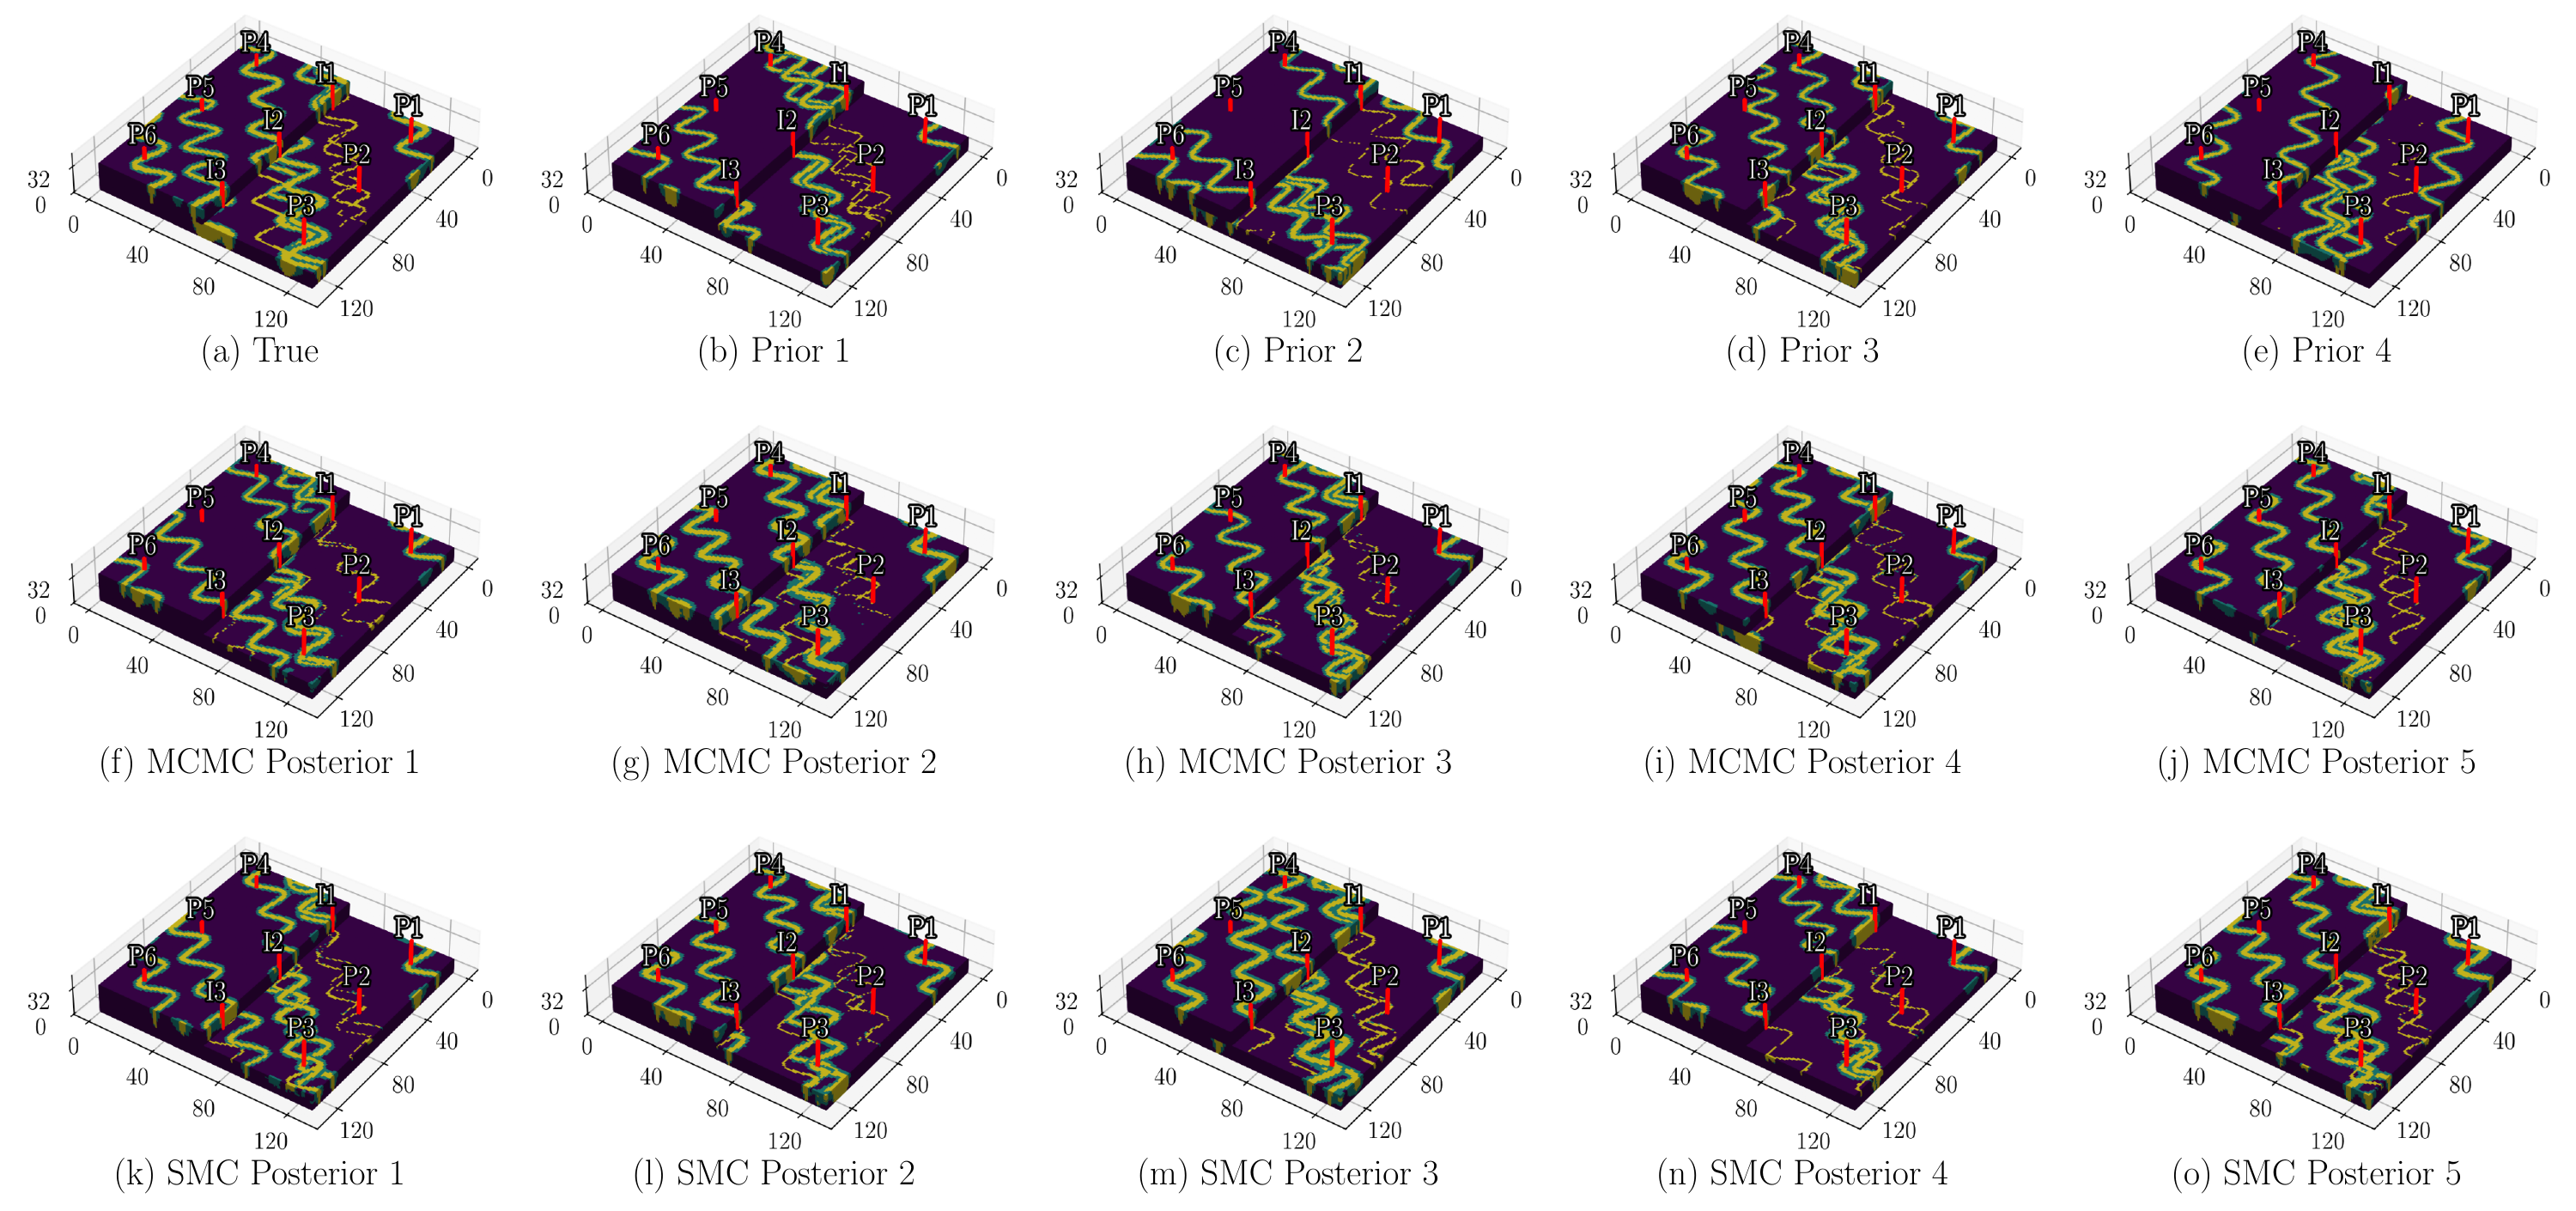}
\caption{Representative 3D facies geomodels for Case~4. Top row shows the true model and four representative prior realizations, and middle and bottom rows show representative MCMC and SMC posterior samples.}
\label{fig:tm104-facies-geomodels}
\end{centeredfigurepage}


\begin{figure}[!htbp]
\centering
\includegraphics[width=0.72\linewidth]{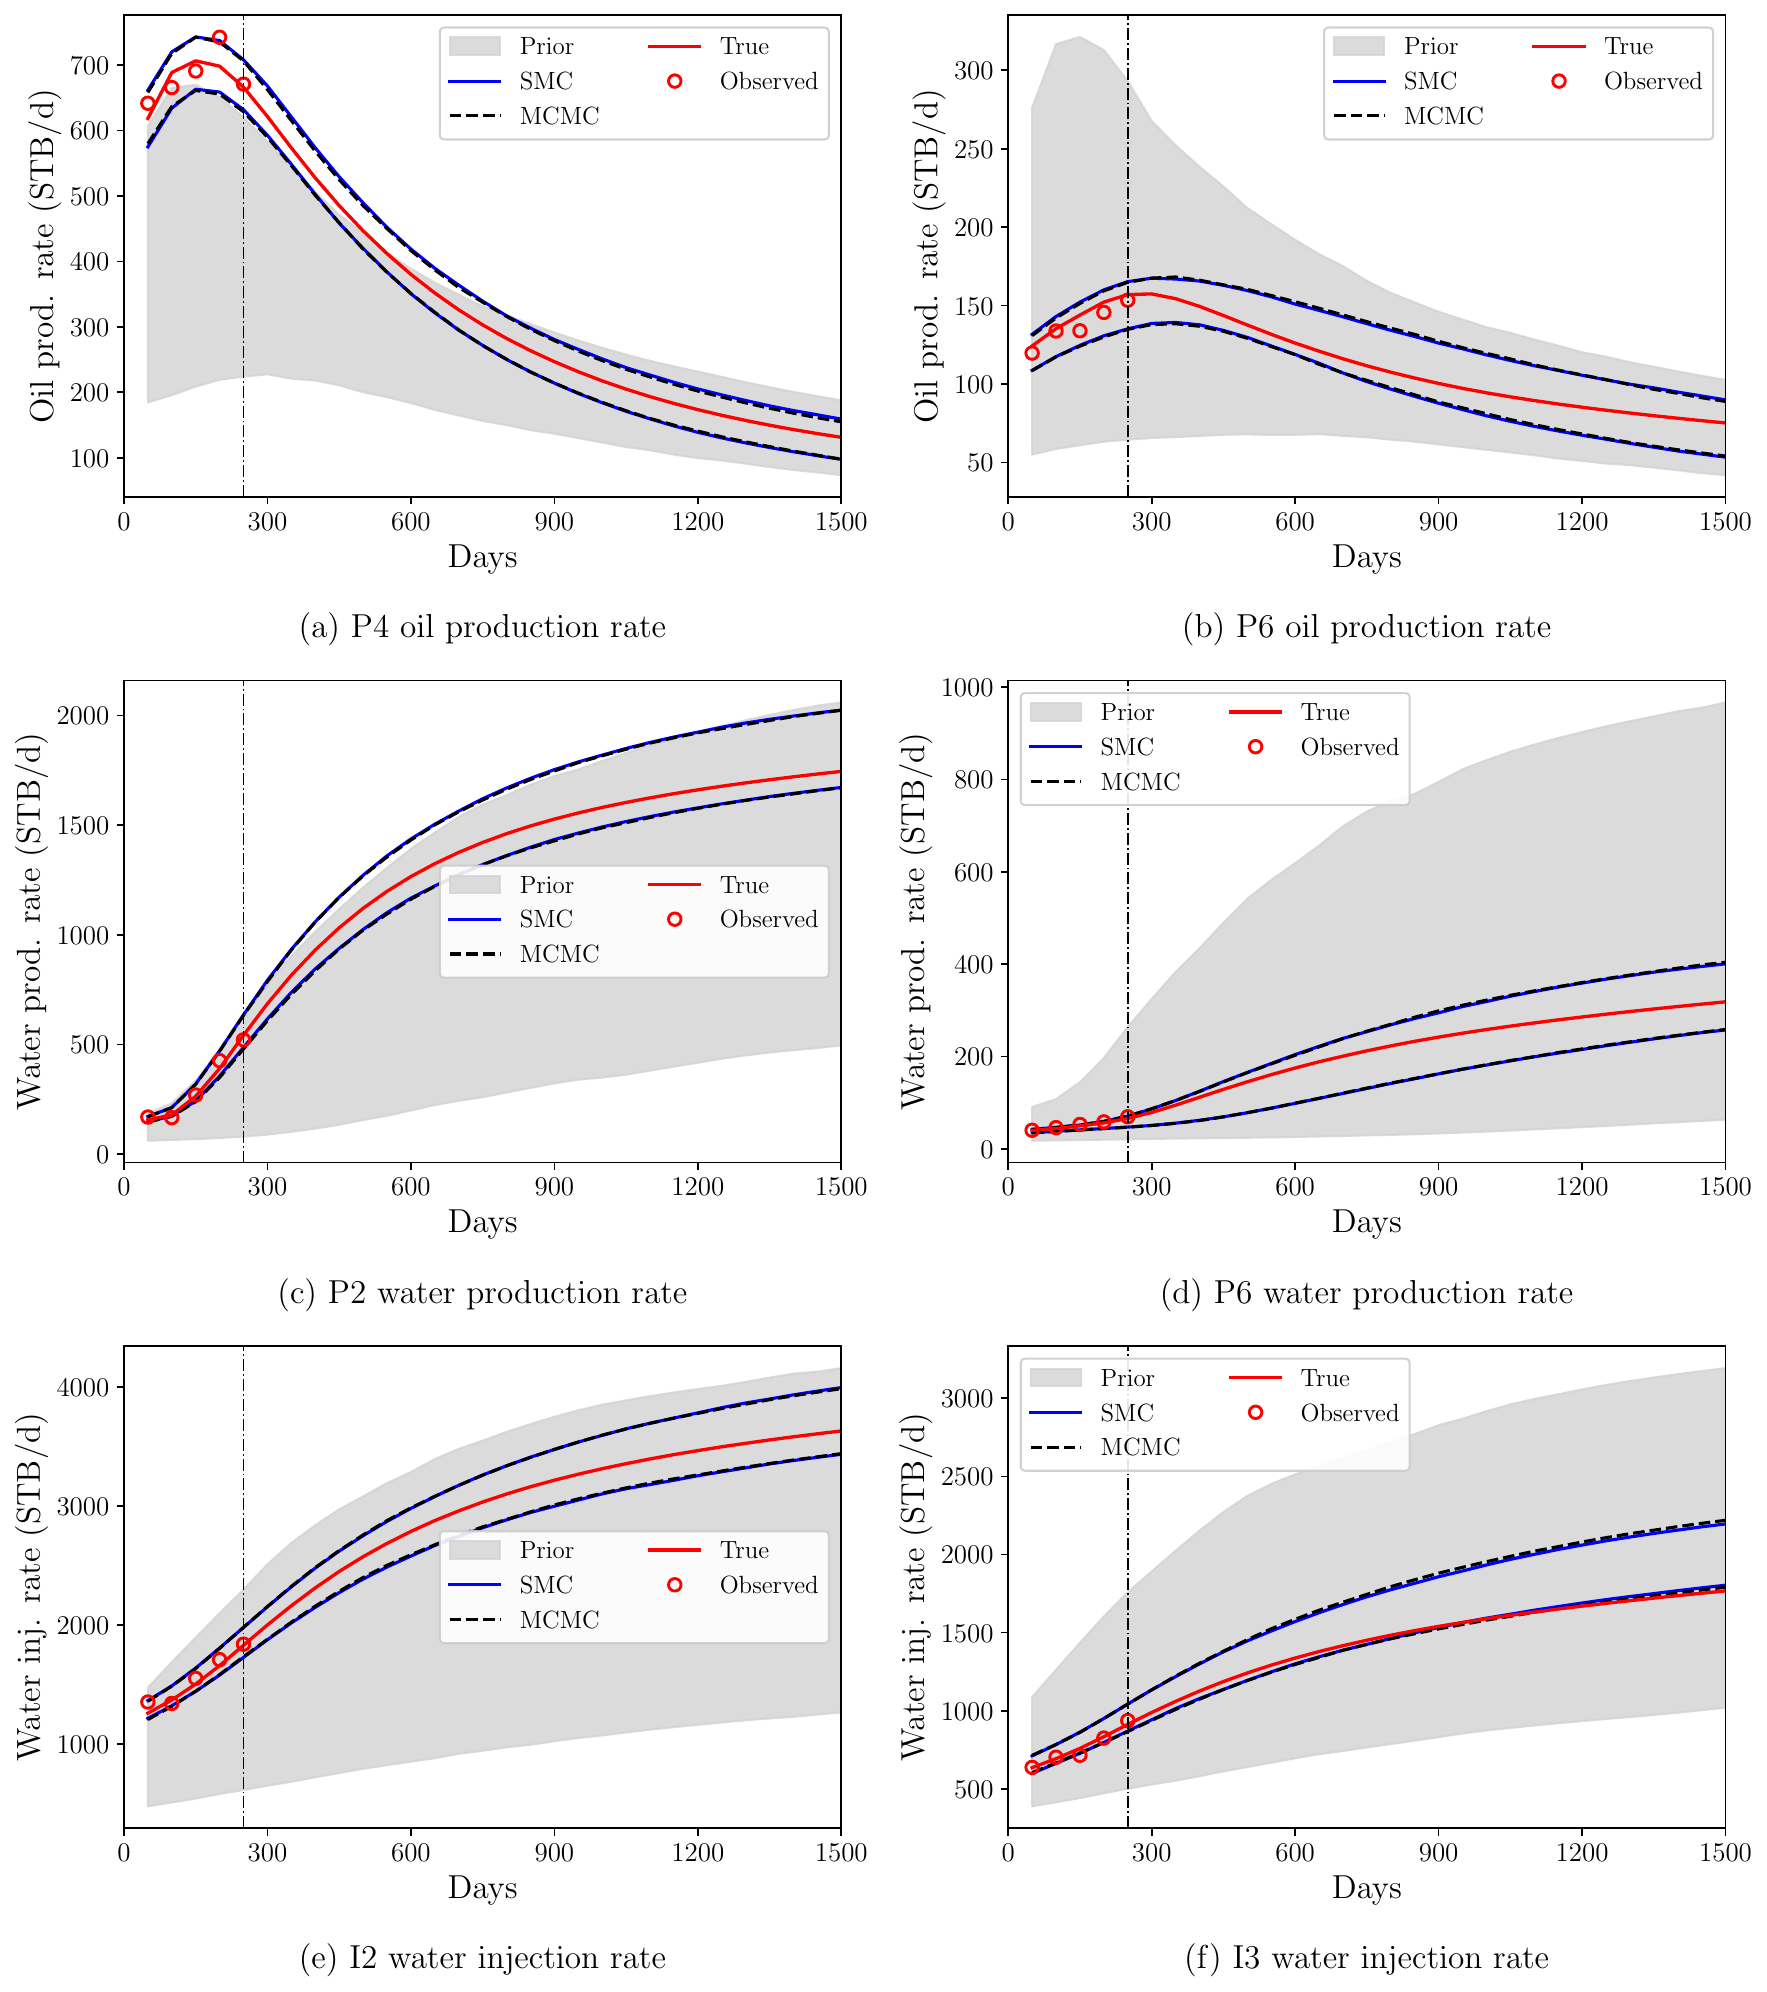}
\caption{Posterior $\mathrm{P}_{10}$--$\mathrm{P}_{90}$ predictions of selected well rates in Case~4. Results are shown for SMC (blue) and MCMC (black dashed), along with the prior $\mathrm{P}_{10}$--$\mathrm{P}_{90}$ range (gray), true response (red), and observed data (red circles). Vertical dashed line indicates the end of the data assimilation time window at 250~days.}
\label{fig:tm104-well-rates}
\end{figure}


\begin{figure}[!htbp]
\centering
\includegraphics[width=0.83\linewidth]{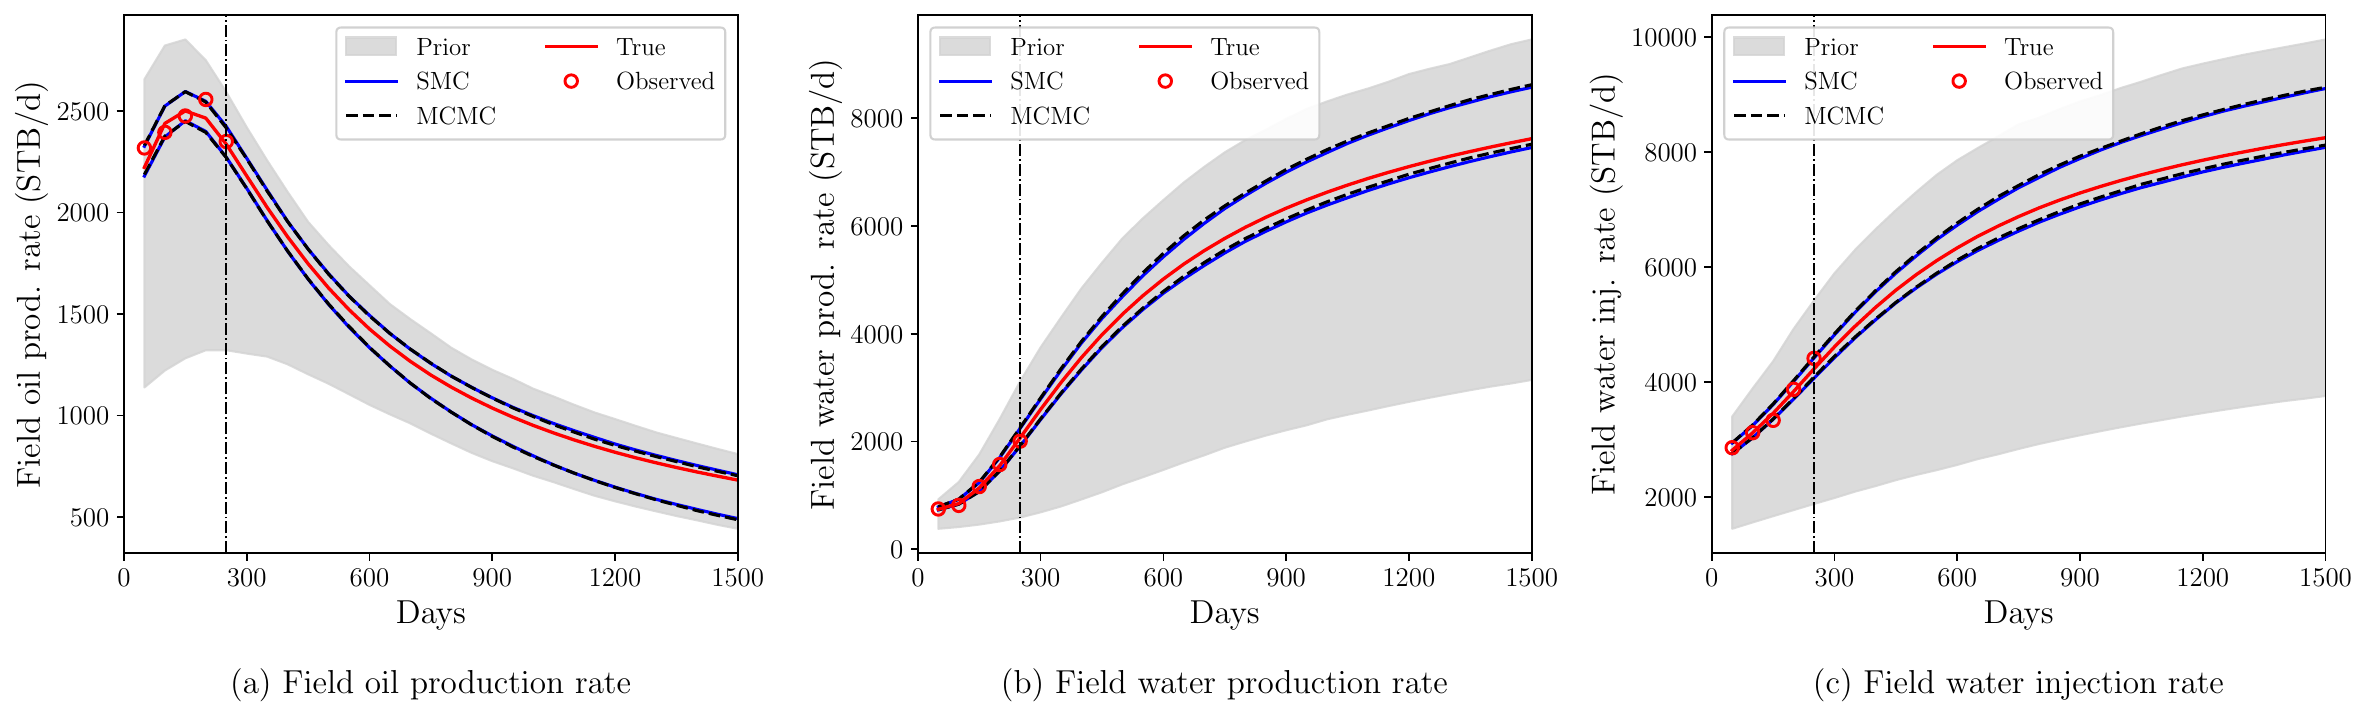}
\caption{Posterior $\mathrm{P}_{10}$--$\mathrm{P}_{90}$ predictions of field rates in Case~4. SMC and MCMC results are shown in blue and black dashed lines, respectively, while the gray regions denote the prior $\mathrm{P}_{10}$--$\mathrm{P}_{90}$ ranges. Red curves represent the true data, and red circles indicate the observed data. The vertical black dashed line marks the end of the data assimilation time window at 250~days.}
\label{fig:tm104-field-rates}
\end{figure}

\end{document}
